# Supplementary material for: Stream-DiffVSR: Low-Latency Streamable Video Super-Resolution via Auto-Regressive Diffusion
Source: arXiv:2512.23709 source file (2026-08-31)

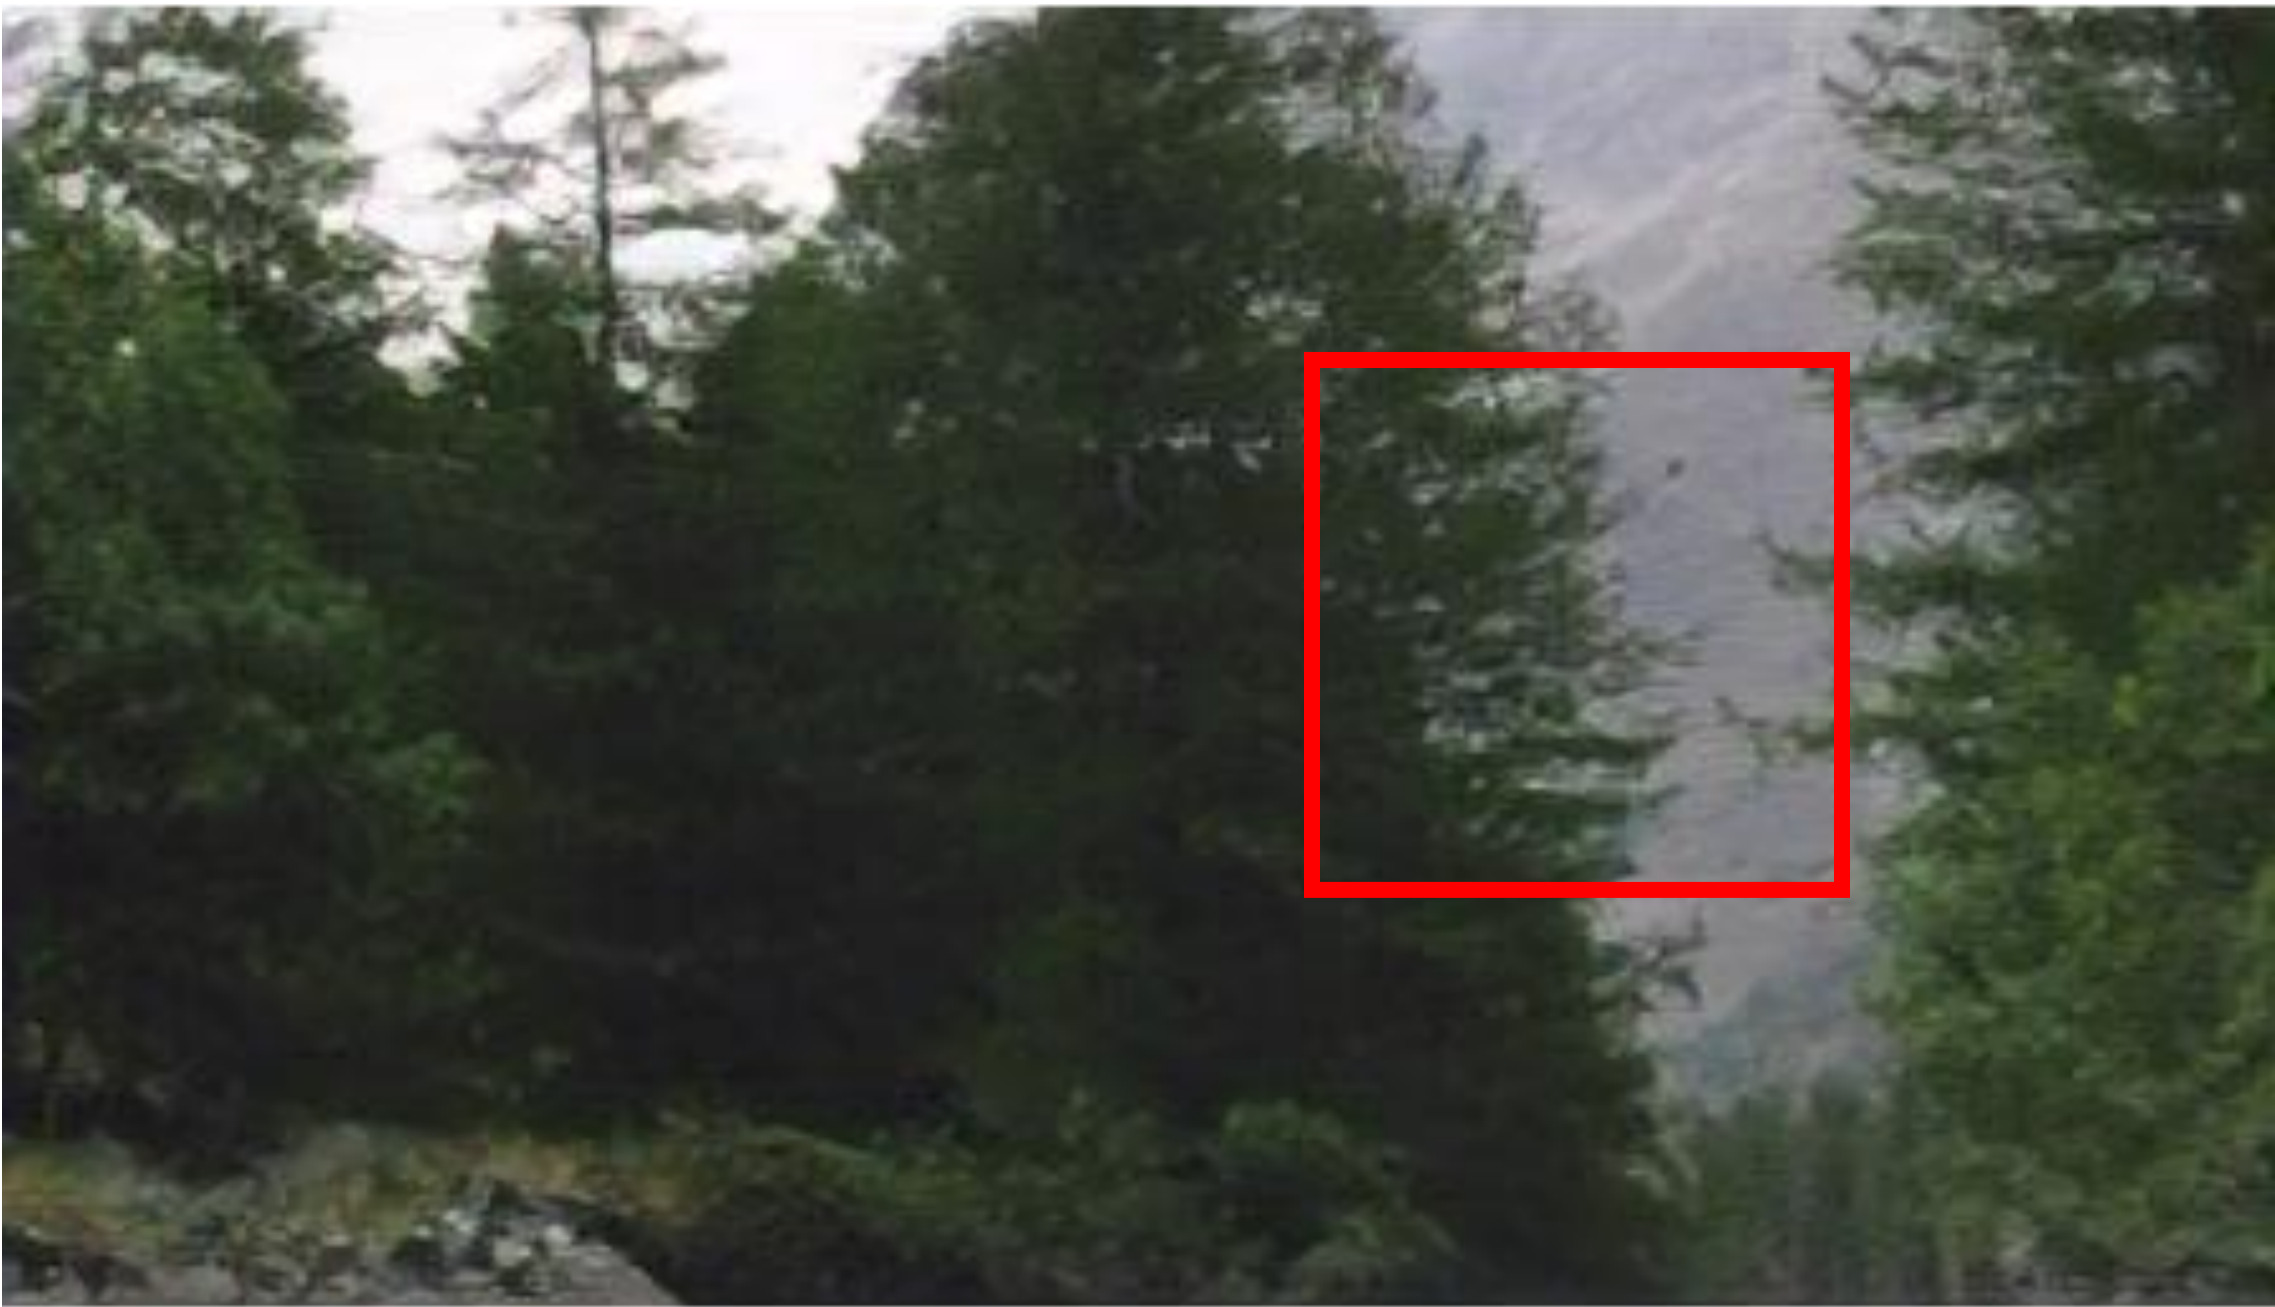

Video frame

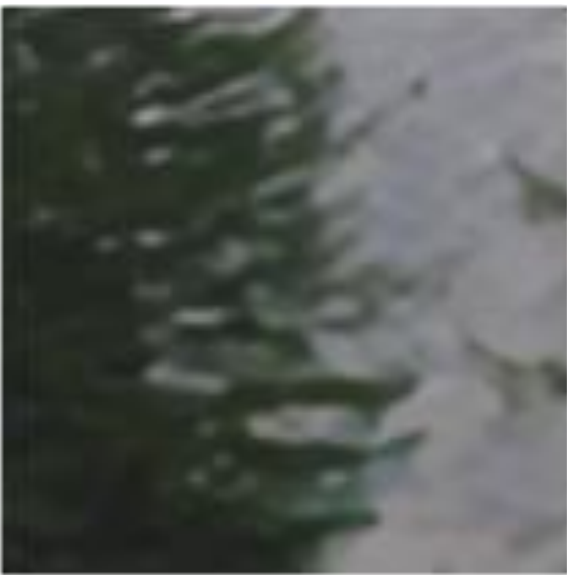

TMP

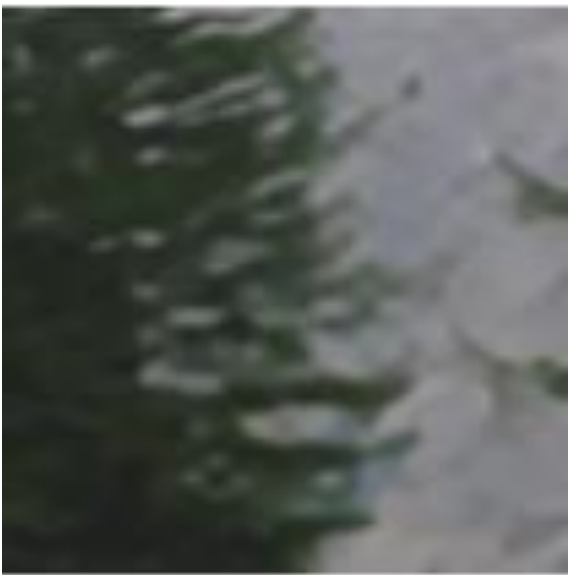

BasicVSR++

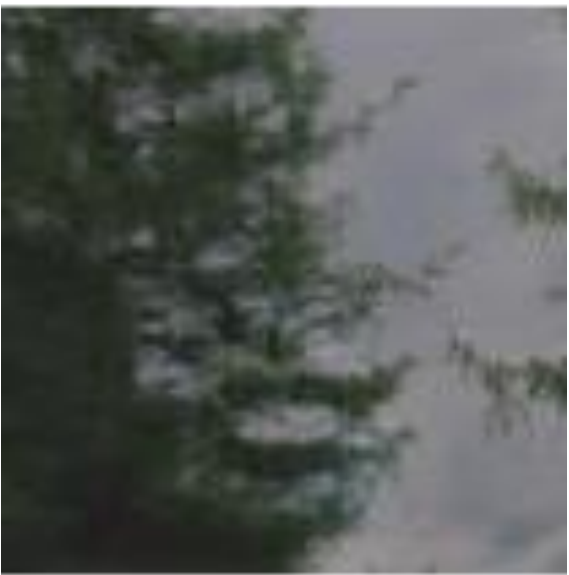

MGLD-VSR

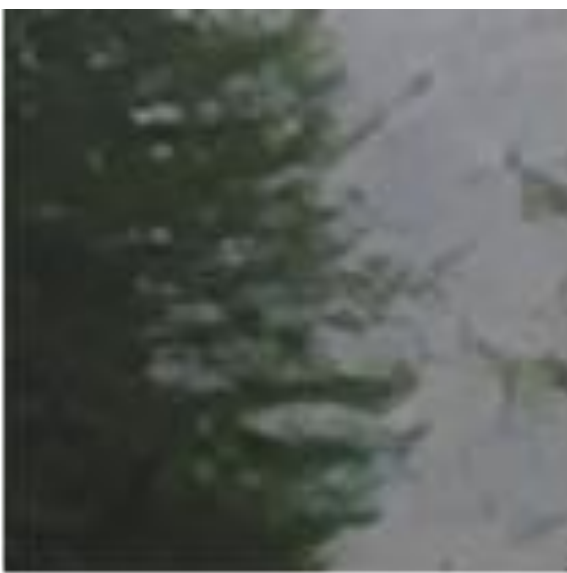

RealViFormer

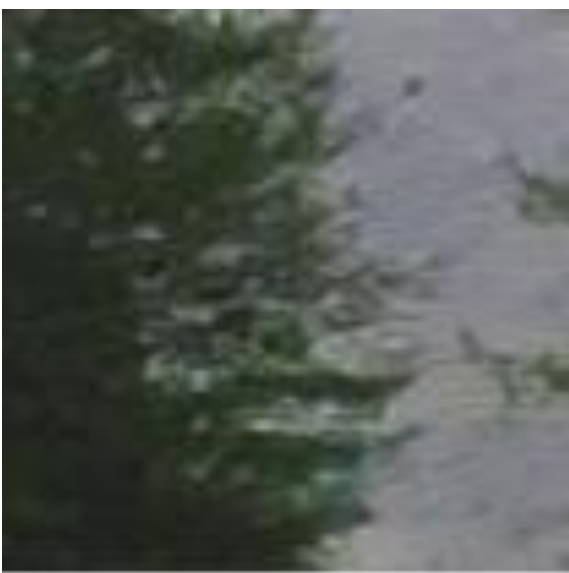

Ours

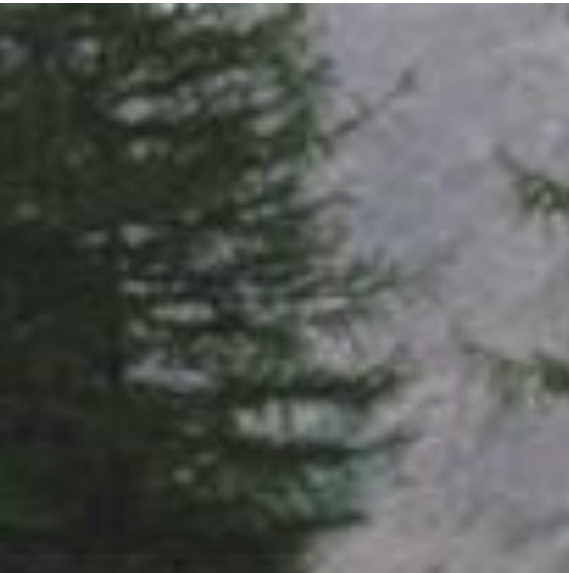

GT

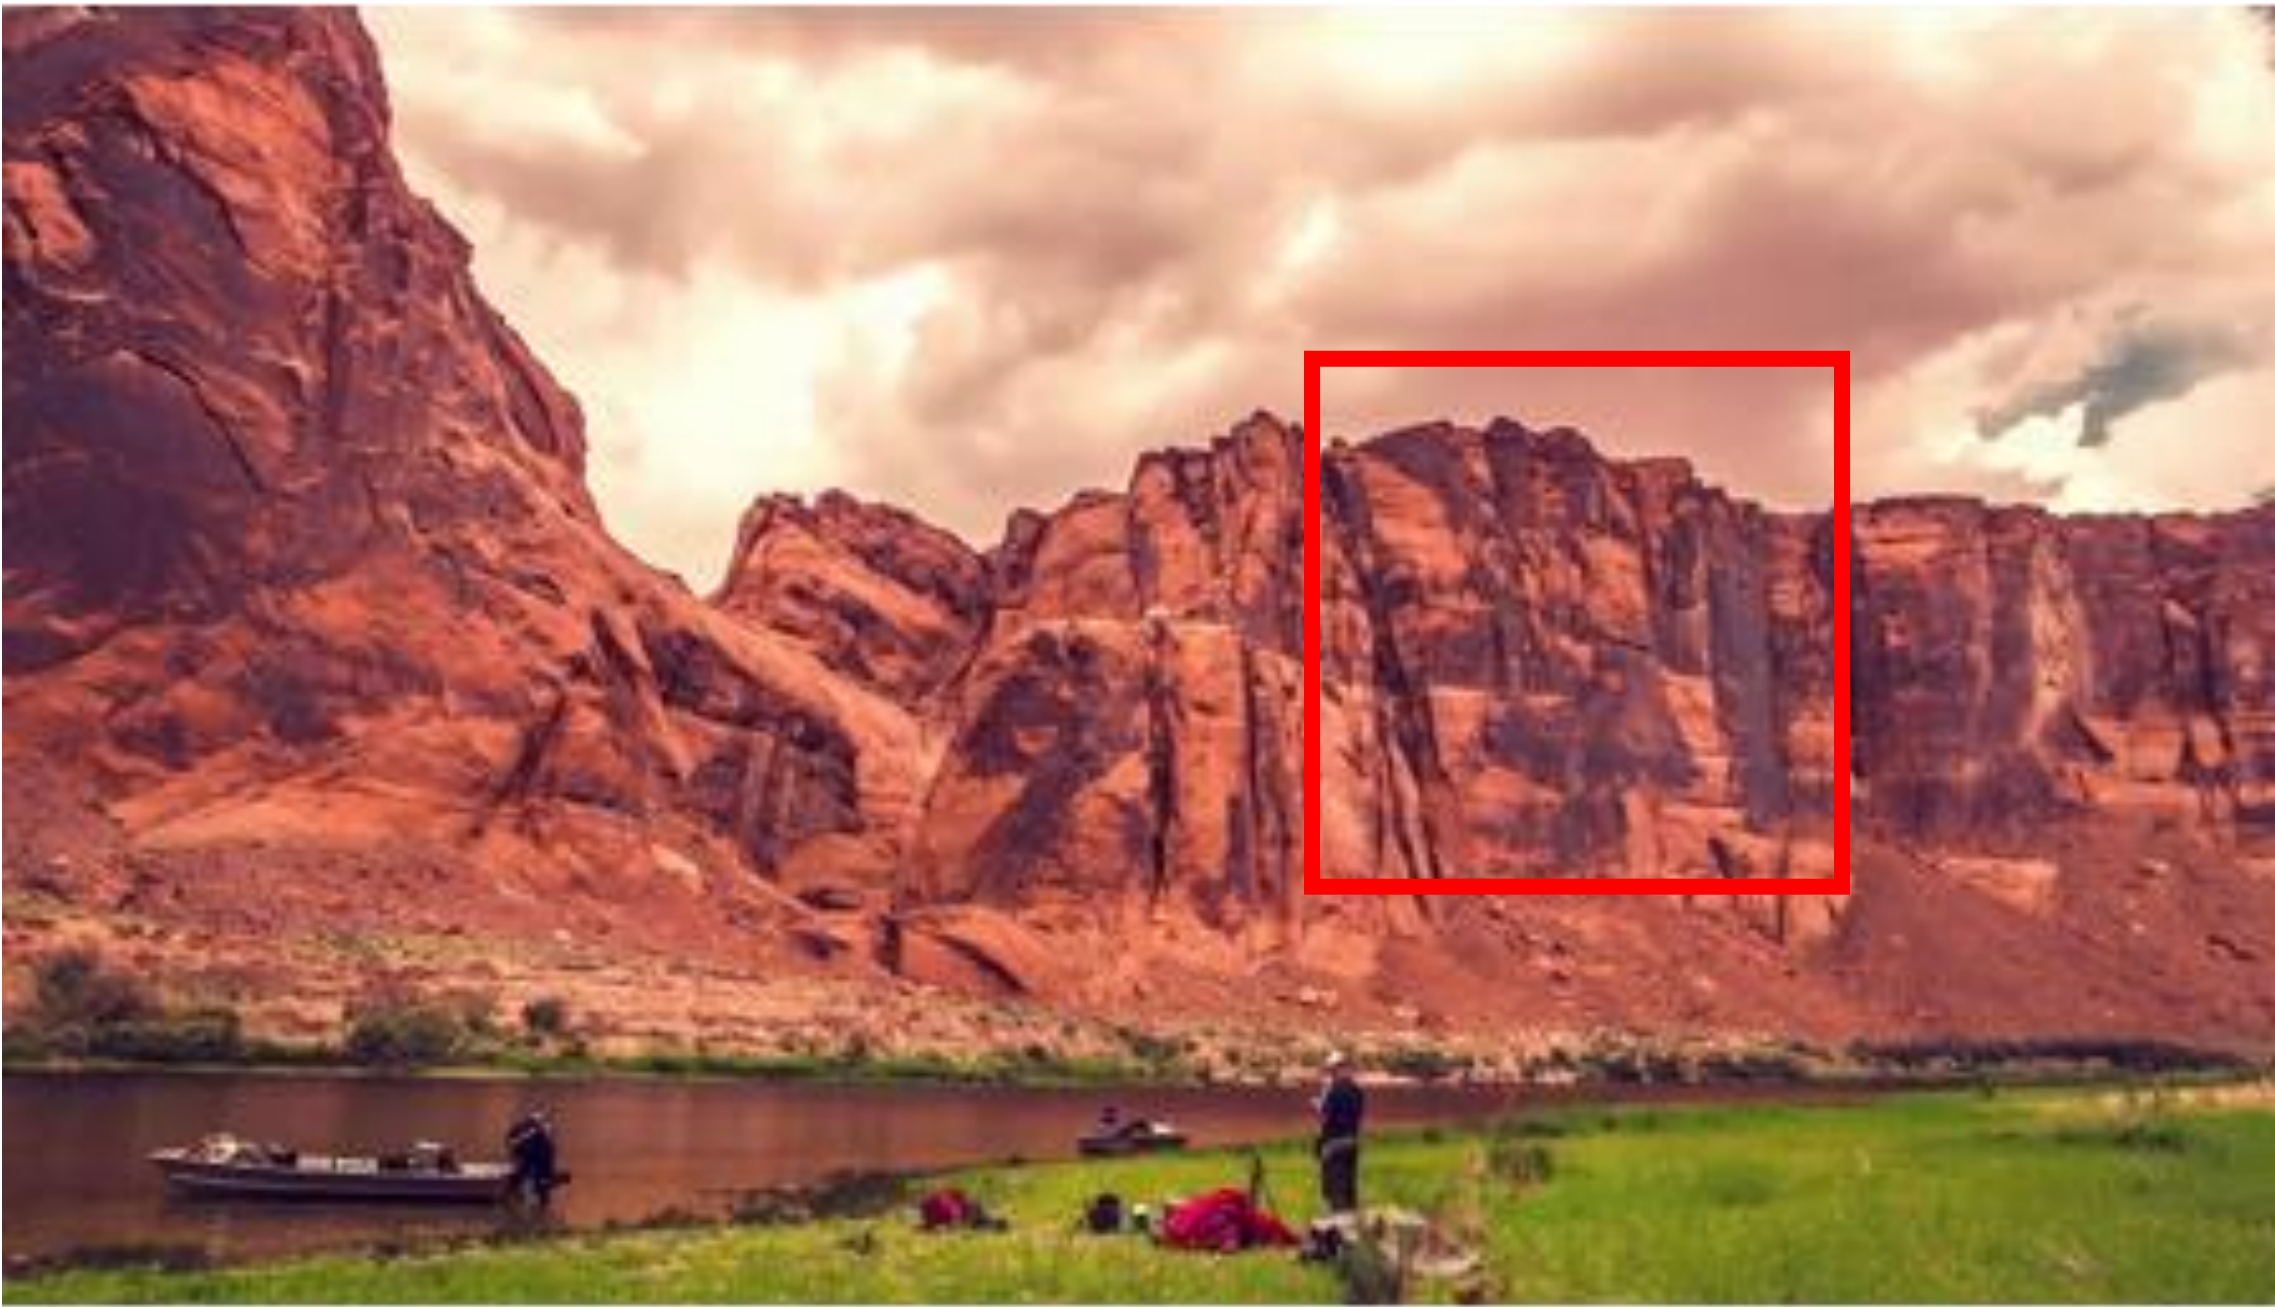

Video frame

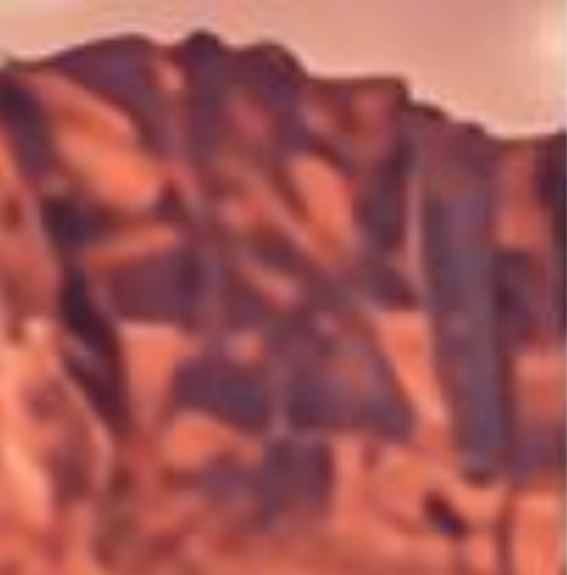

TMP

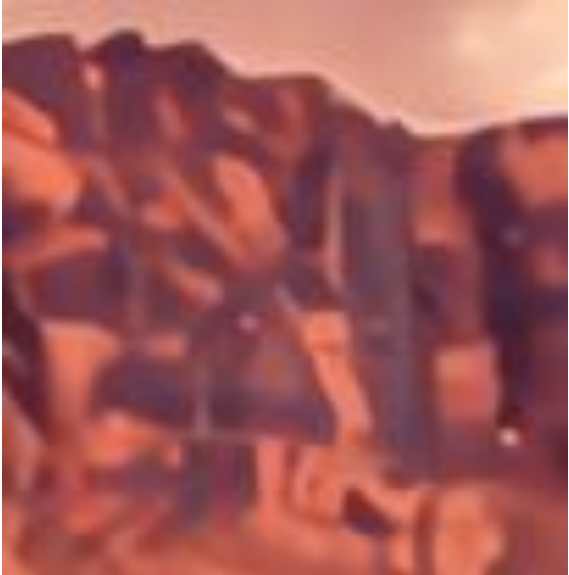

BasicVSR++

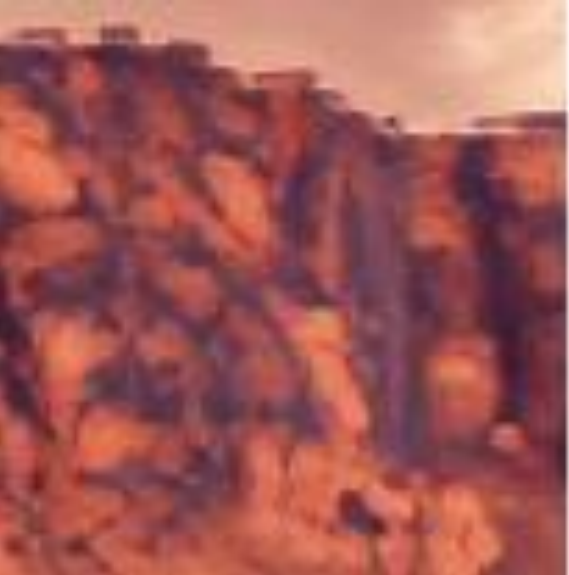

MGLD-VSR

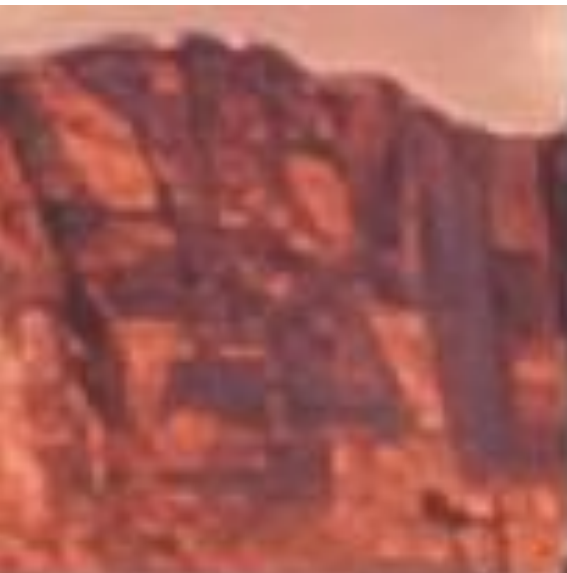

RealViFormer

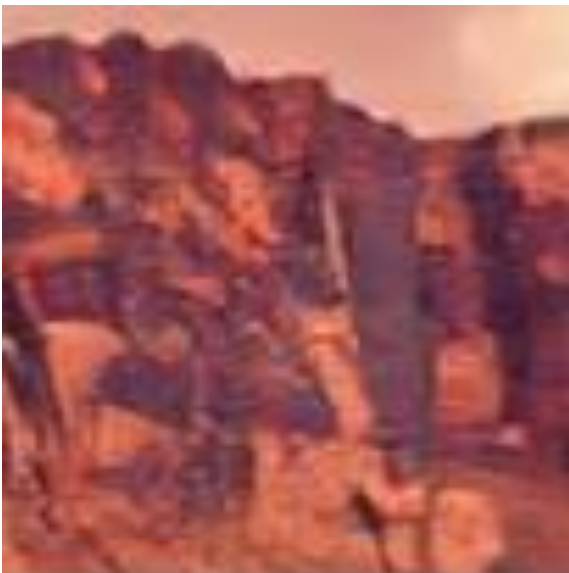

Ours

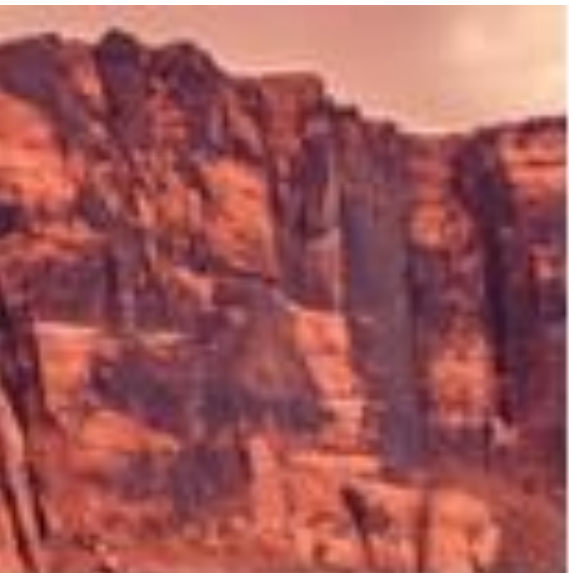

GT

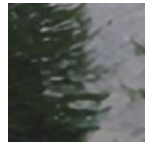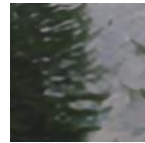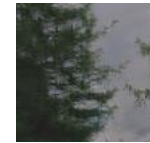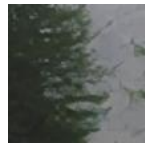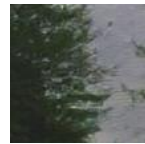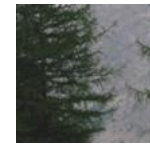

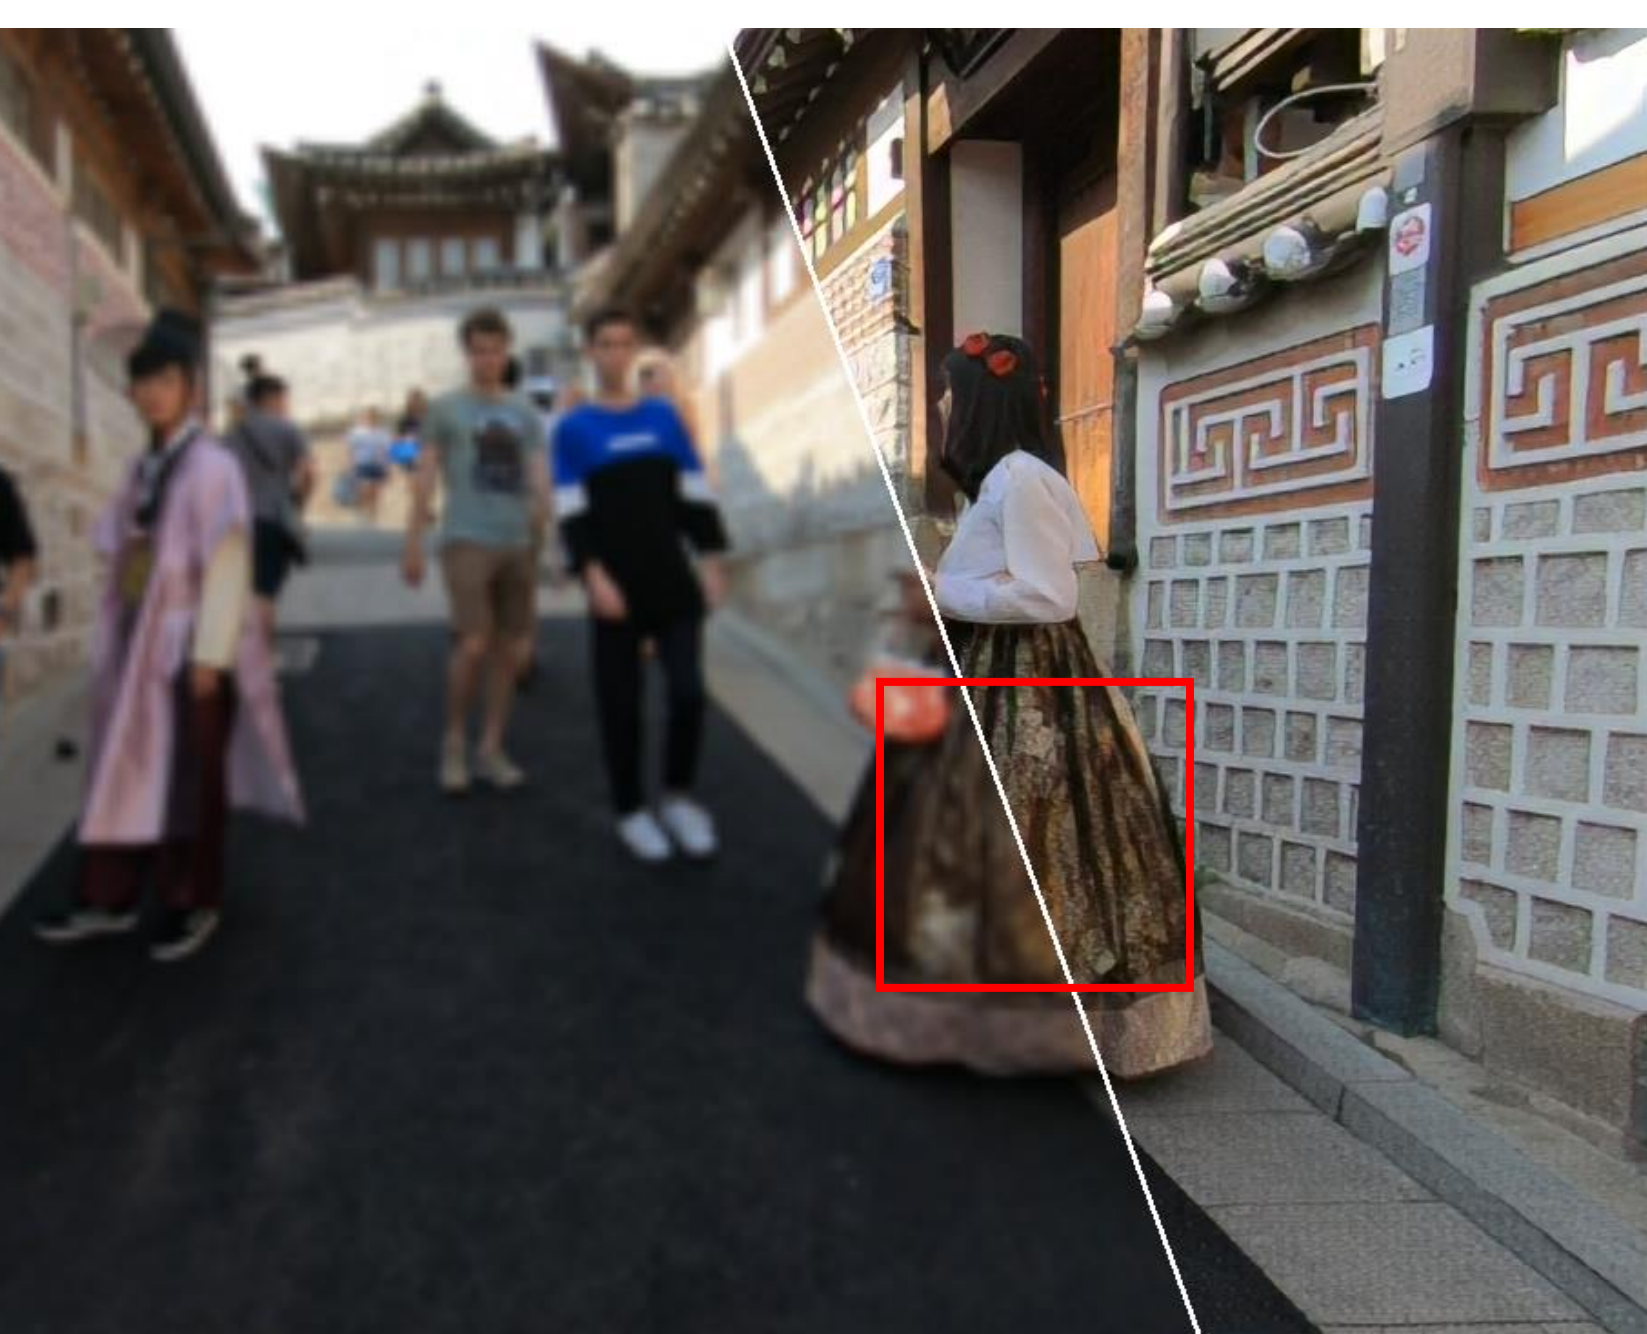

Input/Ours

Bidirectional

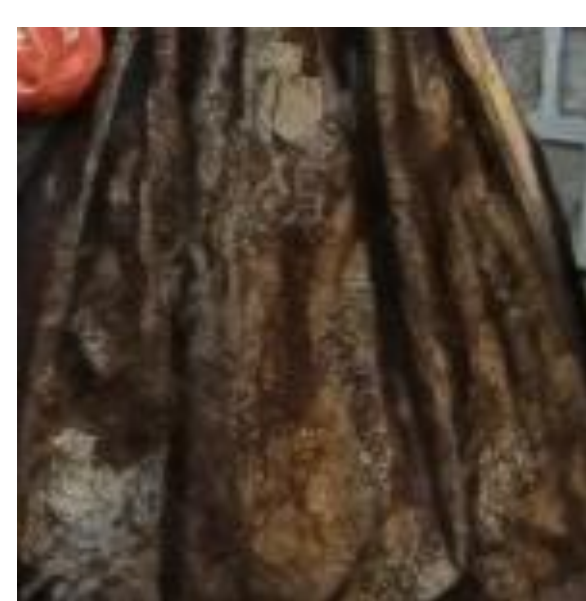

StableVSR

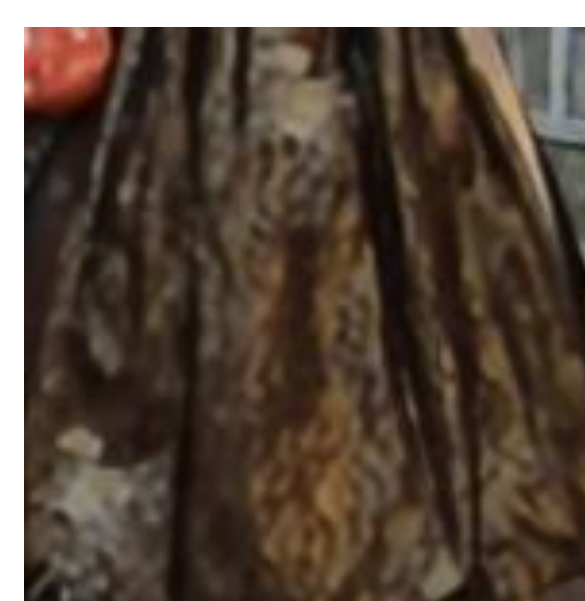

RVRT

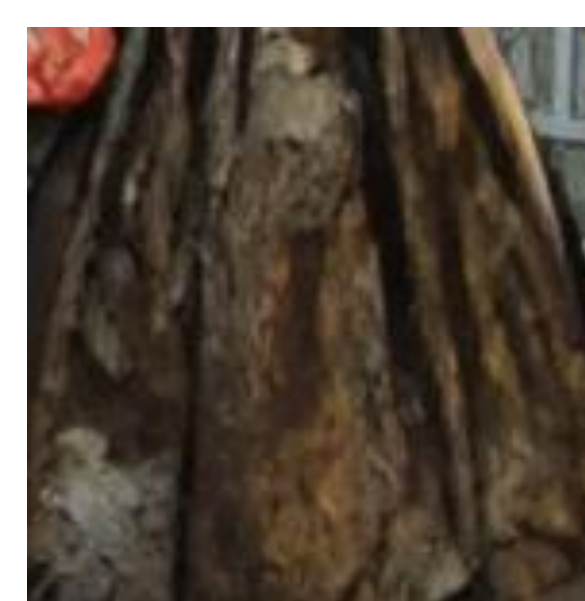

RealBasicVSR

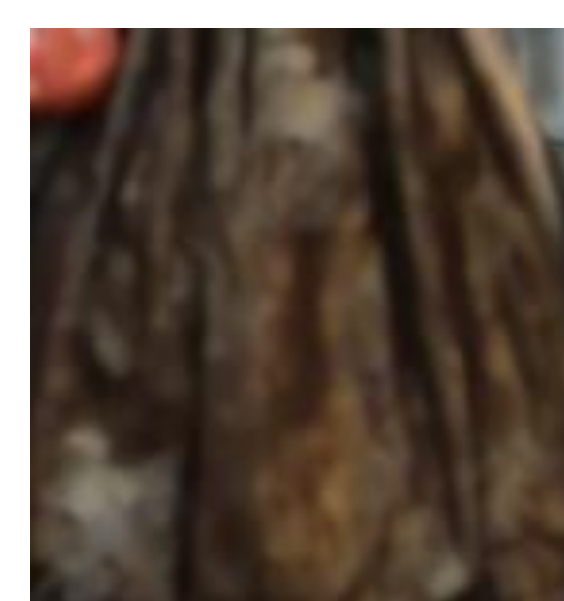

BasicVSR++

Unidirectional

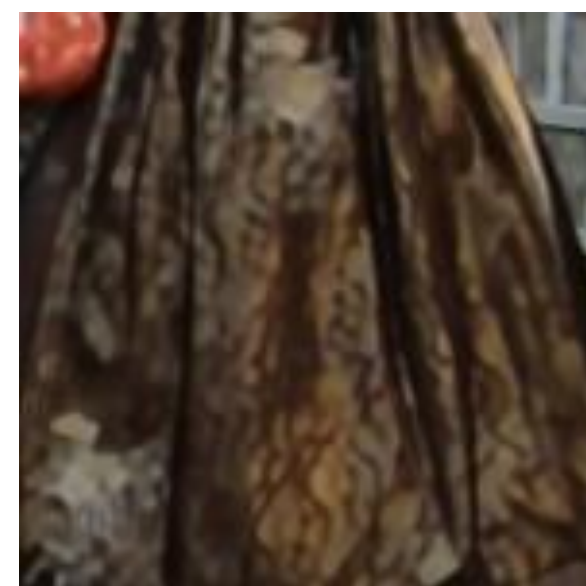

MIA-VSR

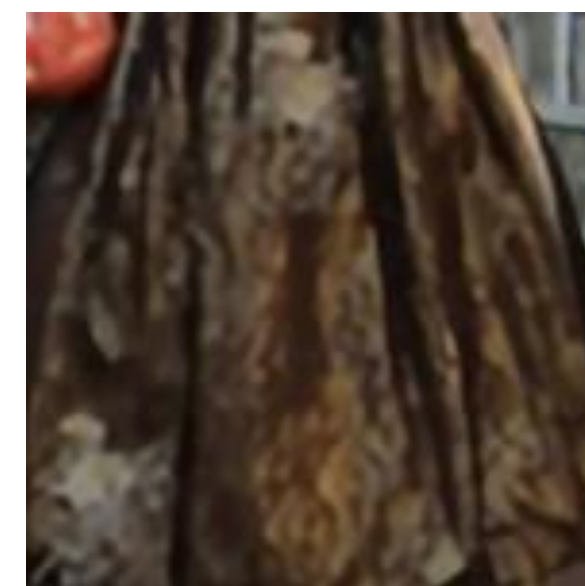

TMP

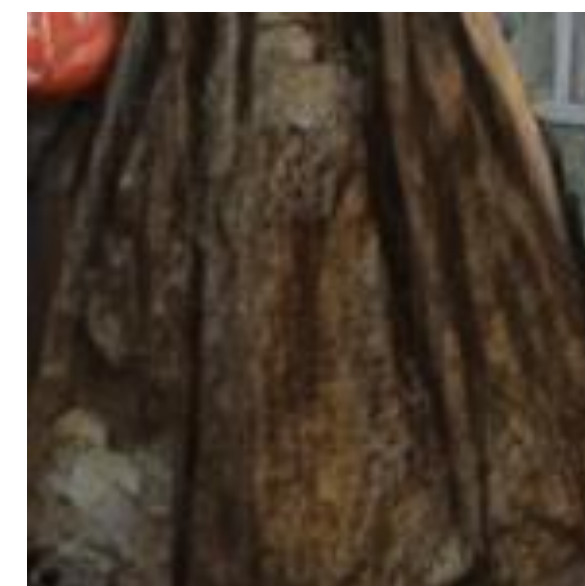

RealViFormer

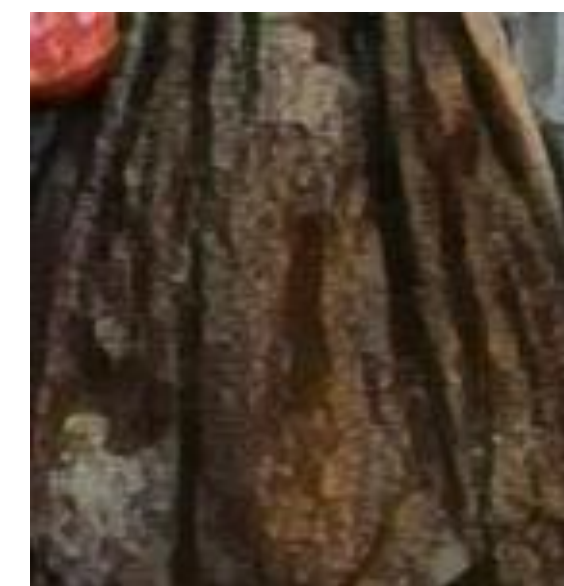

Ours

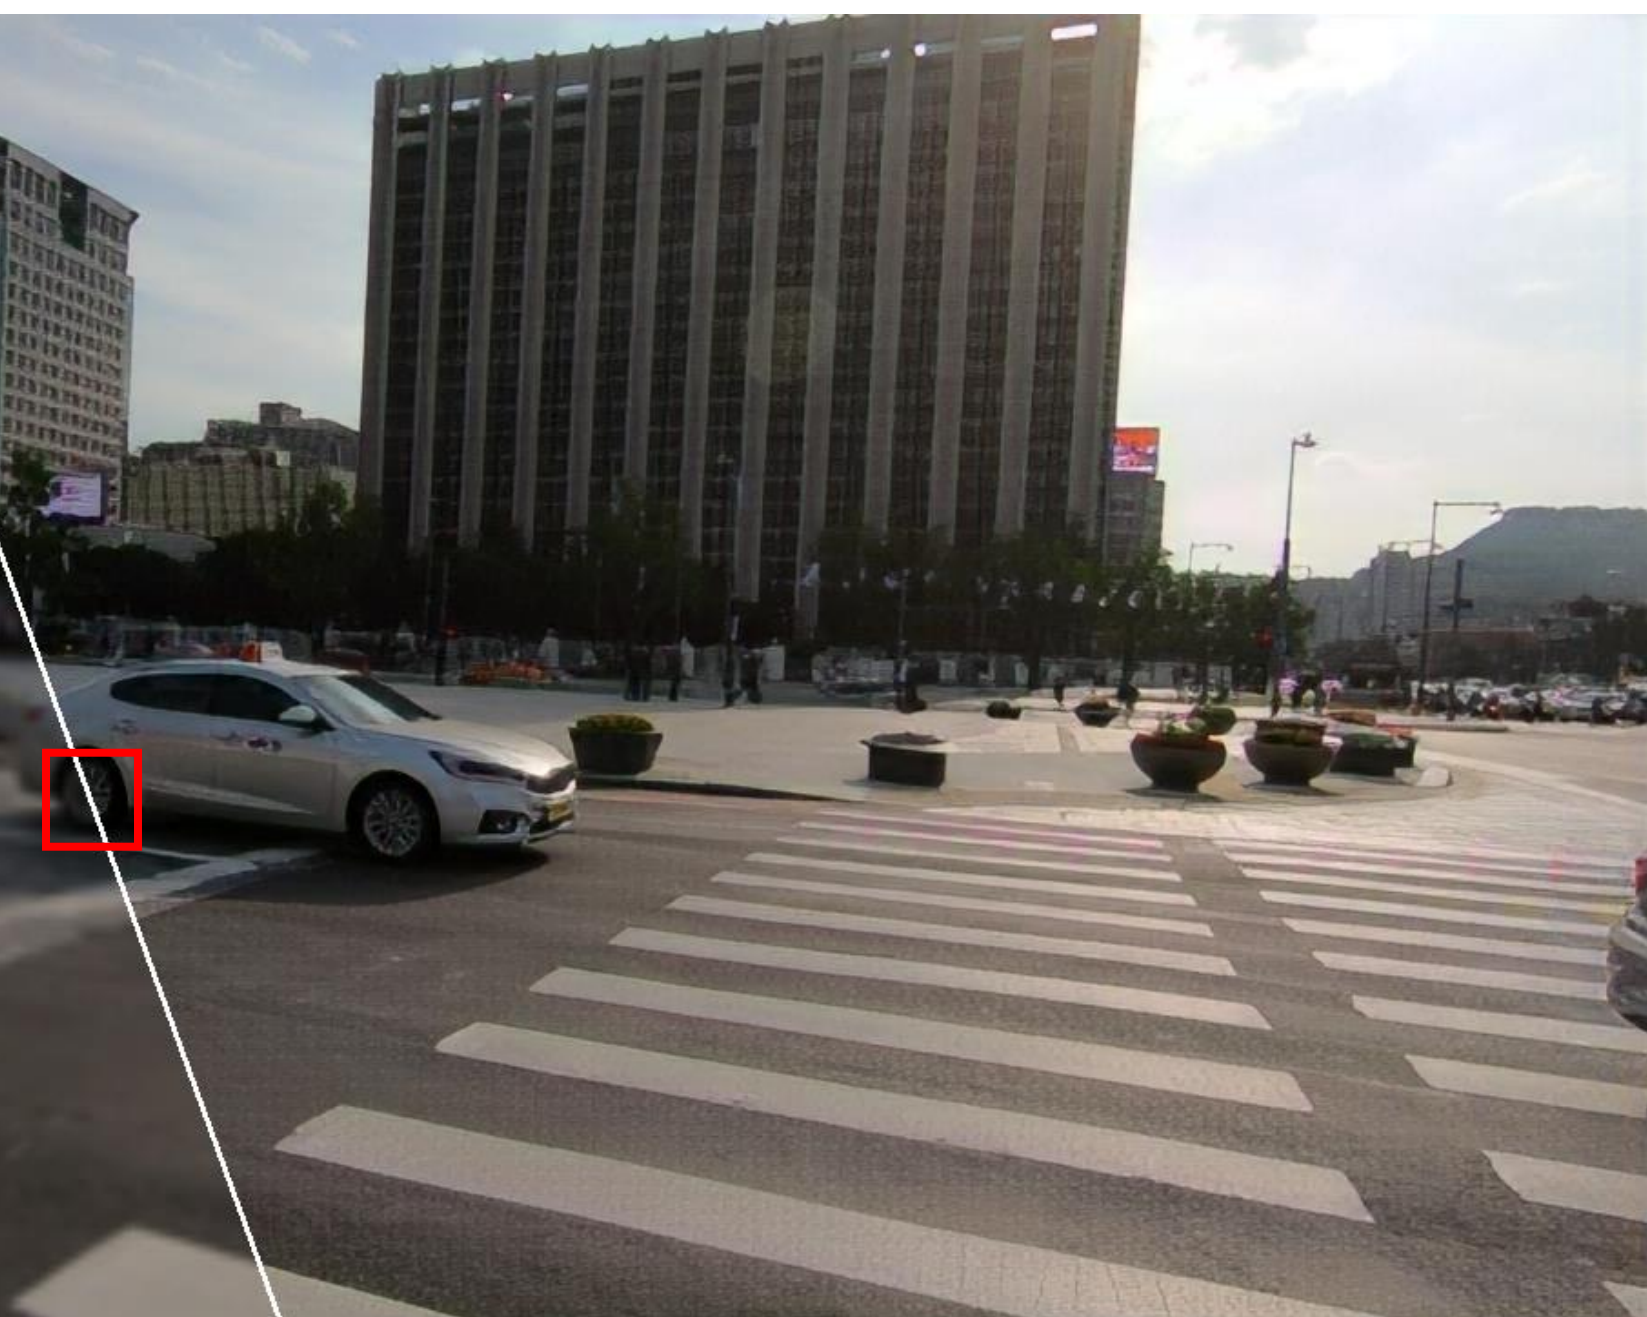

Input/Ours

Bidirectional

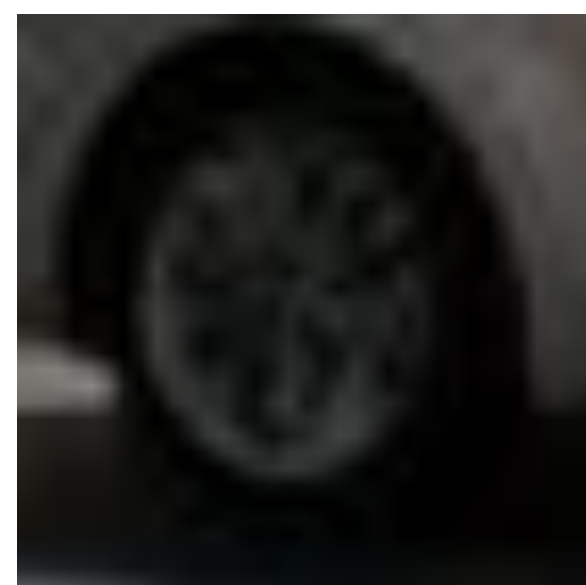

StableVSR

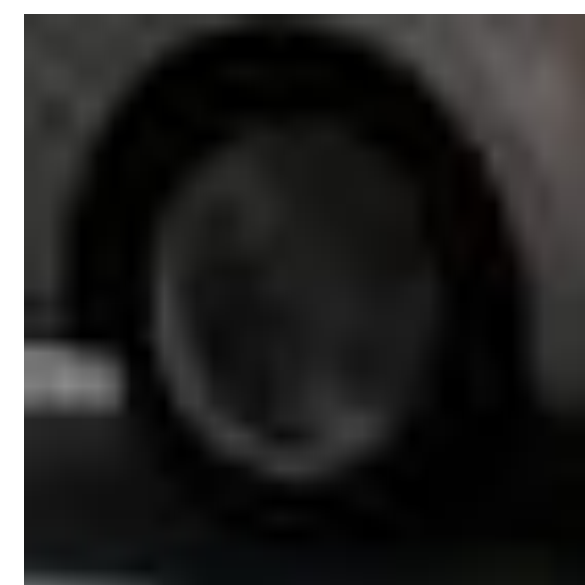

RVRT

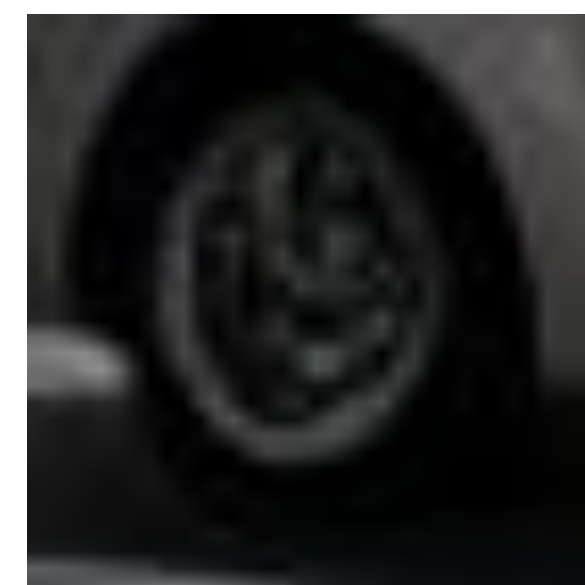

RealBasicVSR

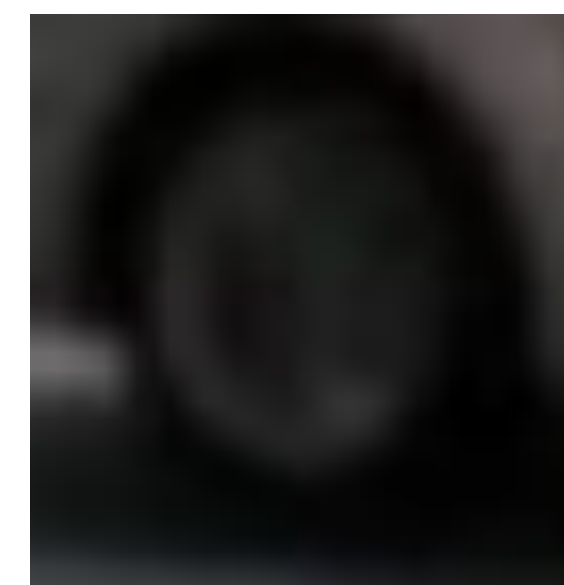

BasicVSR++

Unidirectional

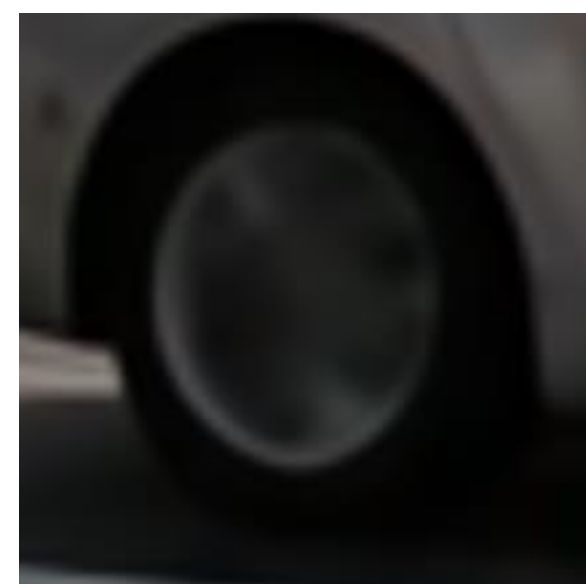

MIA-VSR

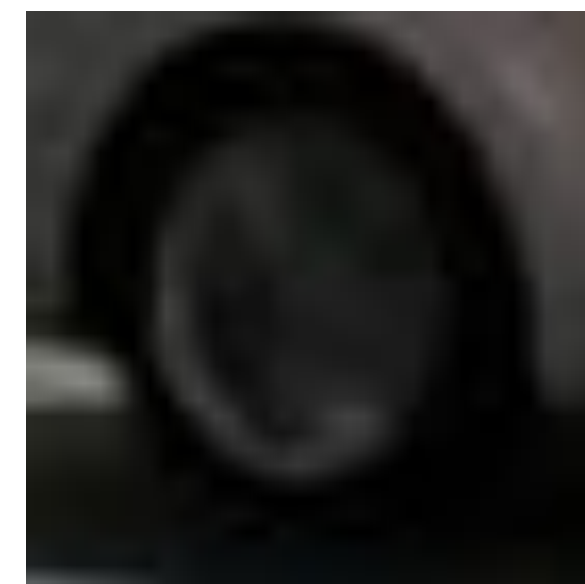

TMP

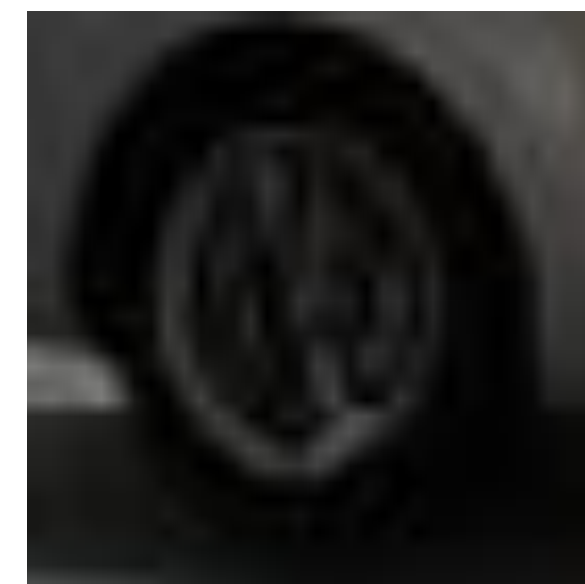

RealViFormer

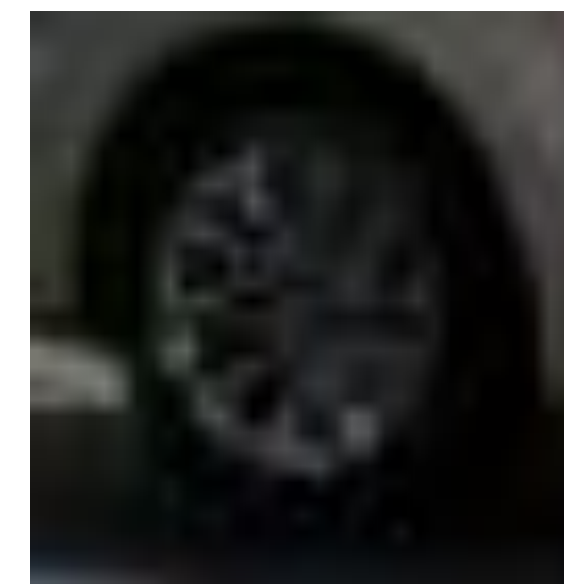

Ours

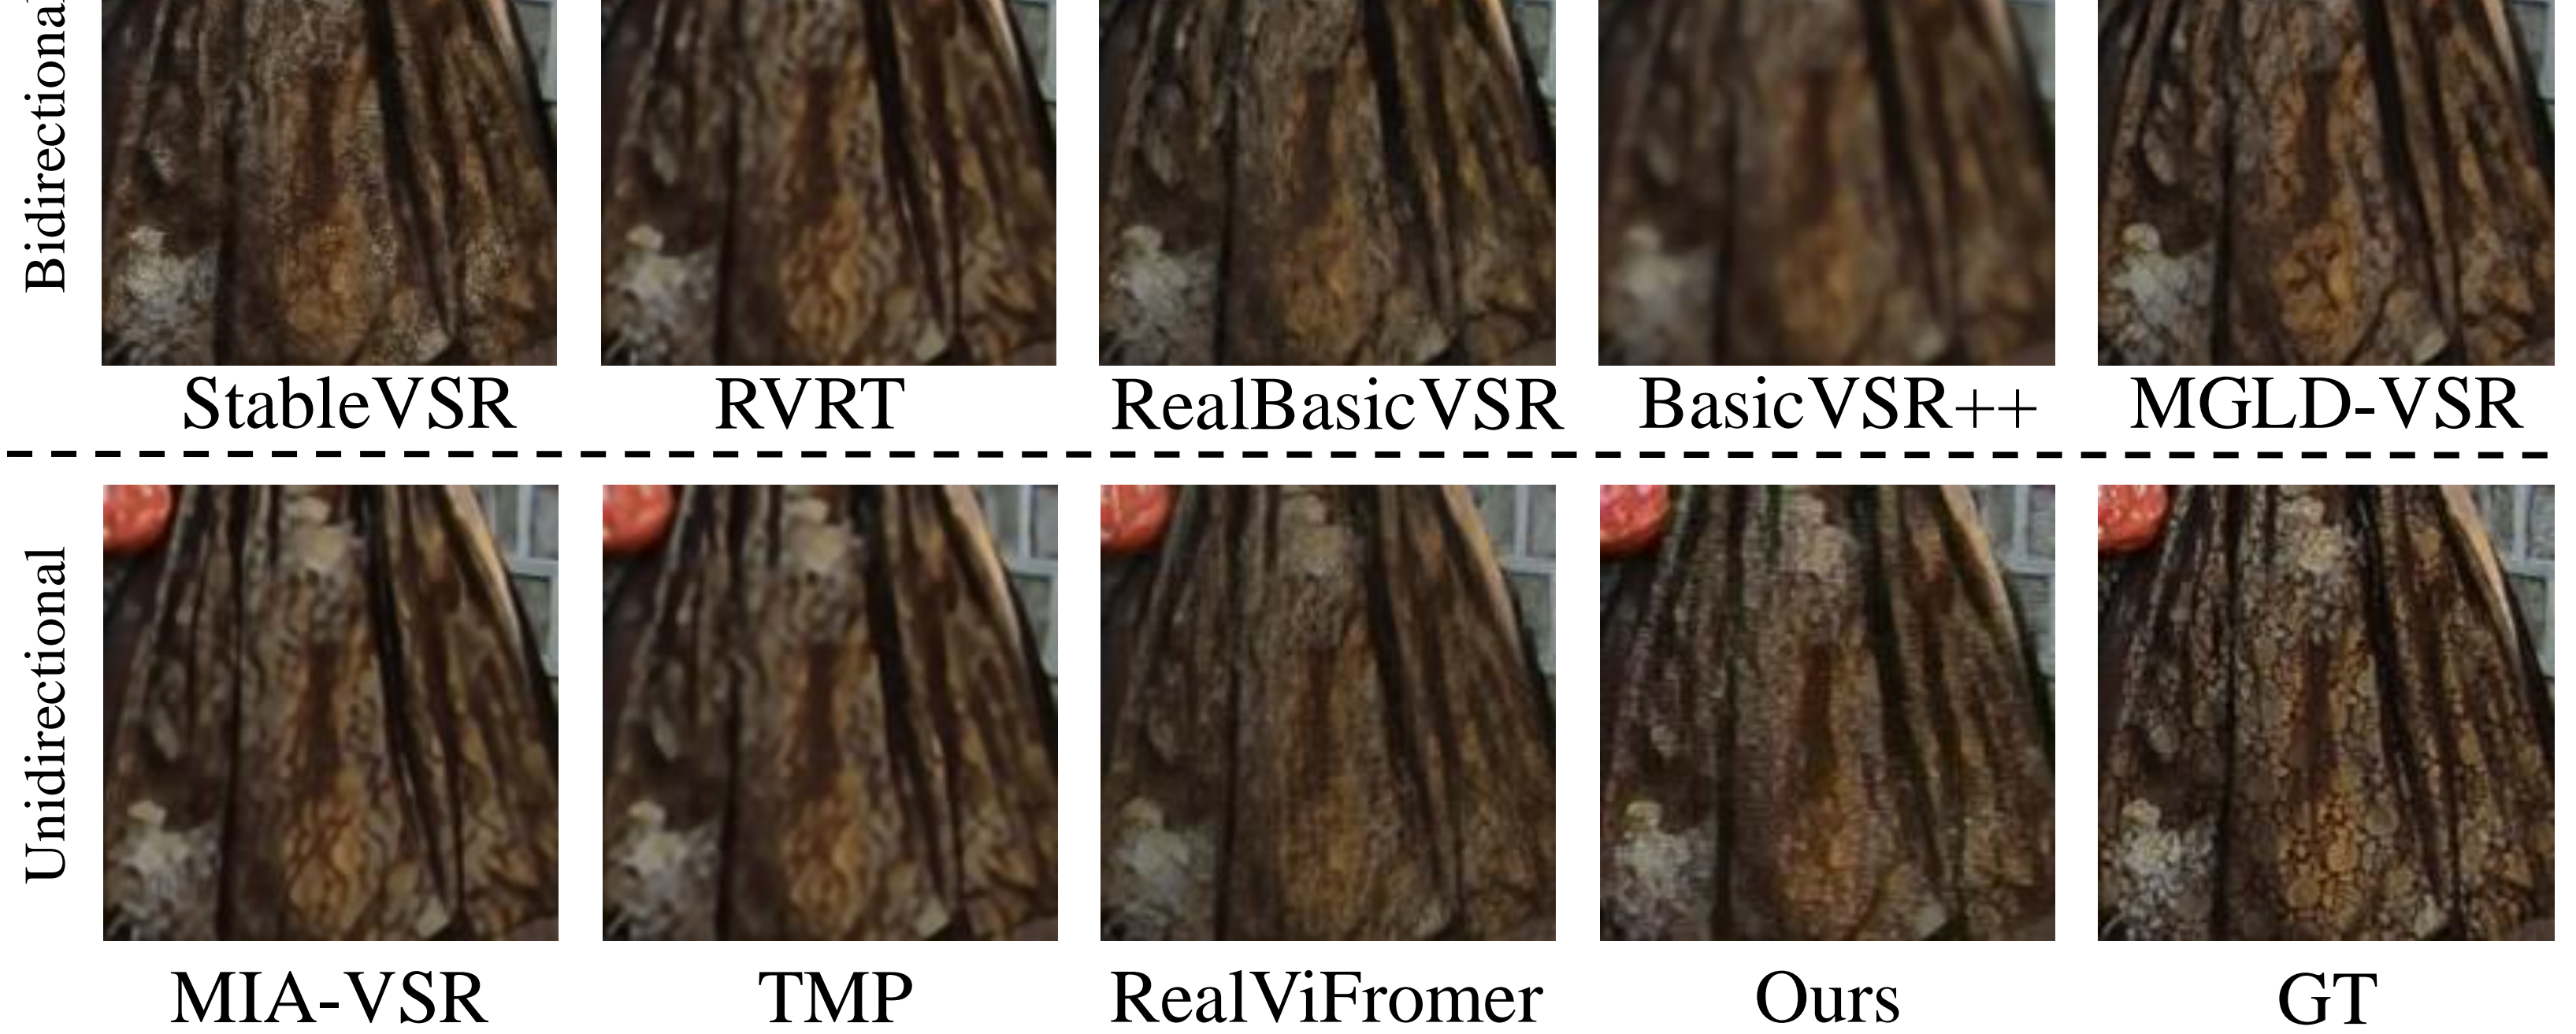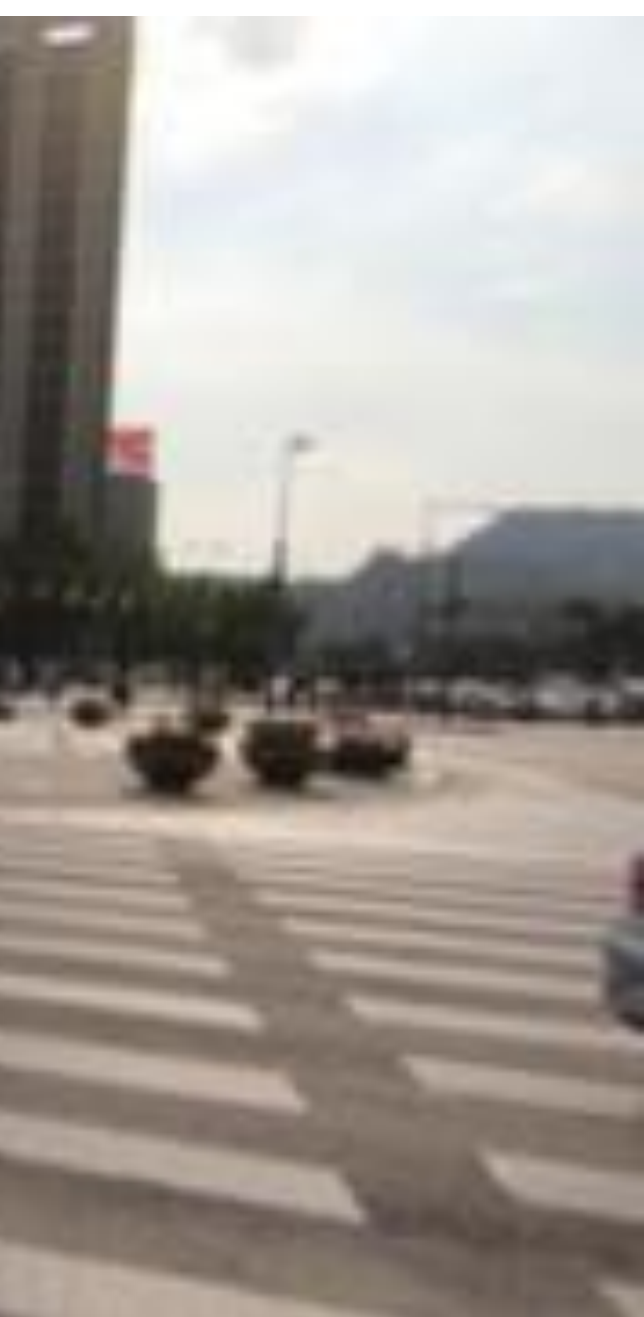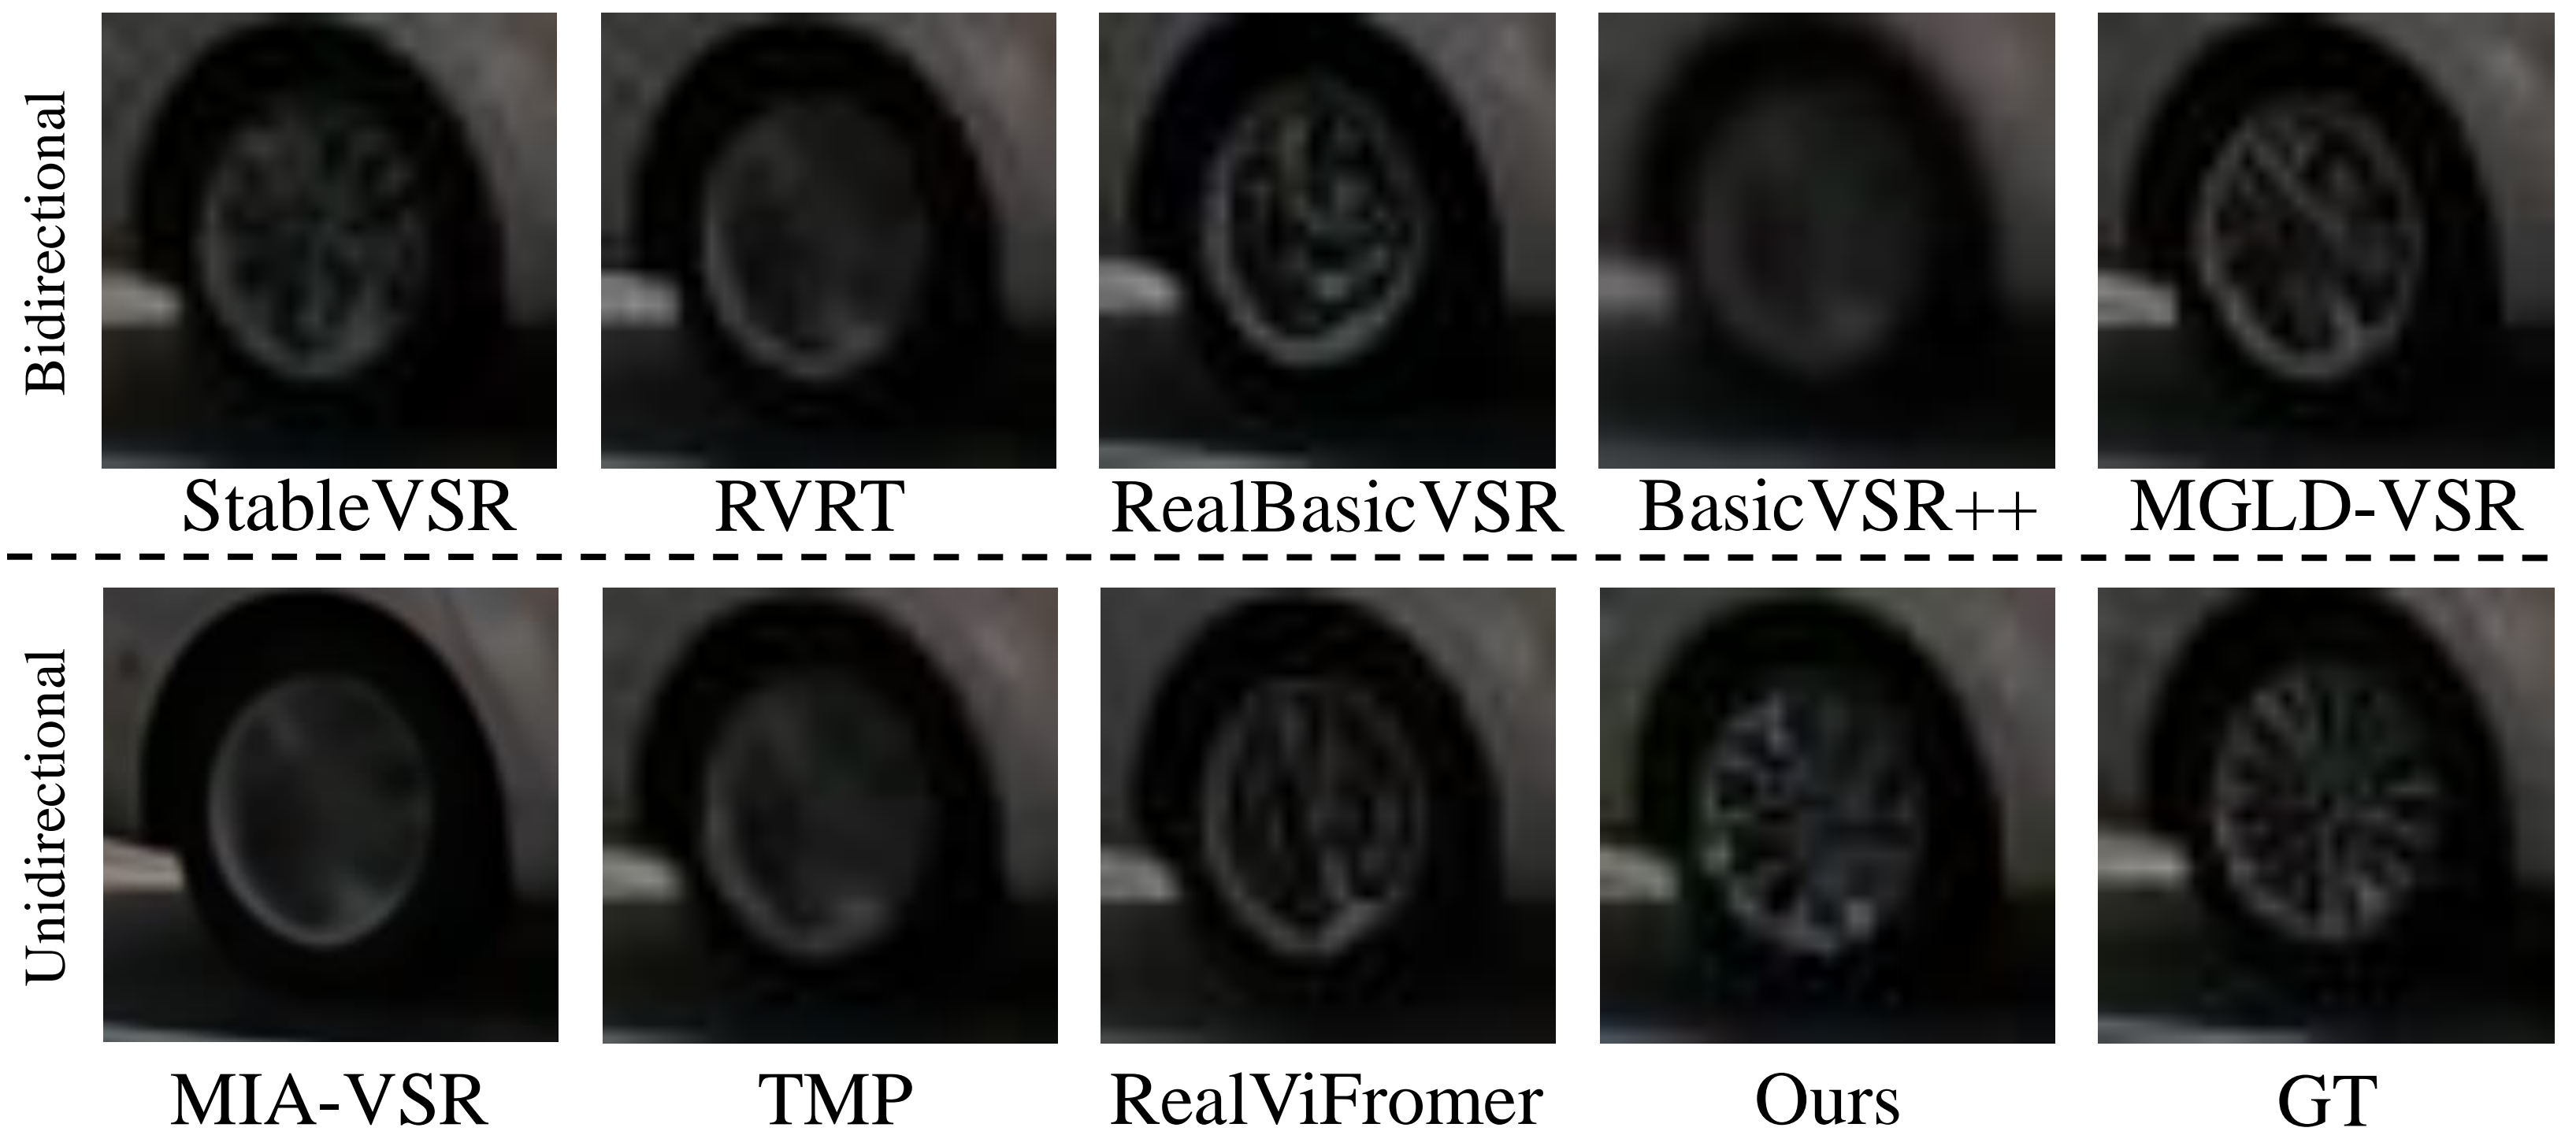

Supplement: Supplementary file 1 [file suppl_v1.pdf]
