# Supplementary material for: Stream-DiffVSR: Low-Latency Streamable Video Super-Resolution via Auto-Regressive Diffusion
Source: arXiv:2512.23709 source file (2026-08-31)

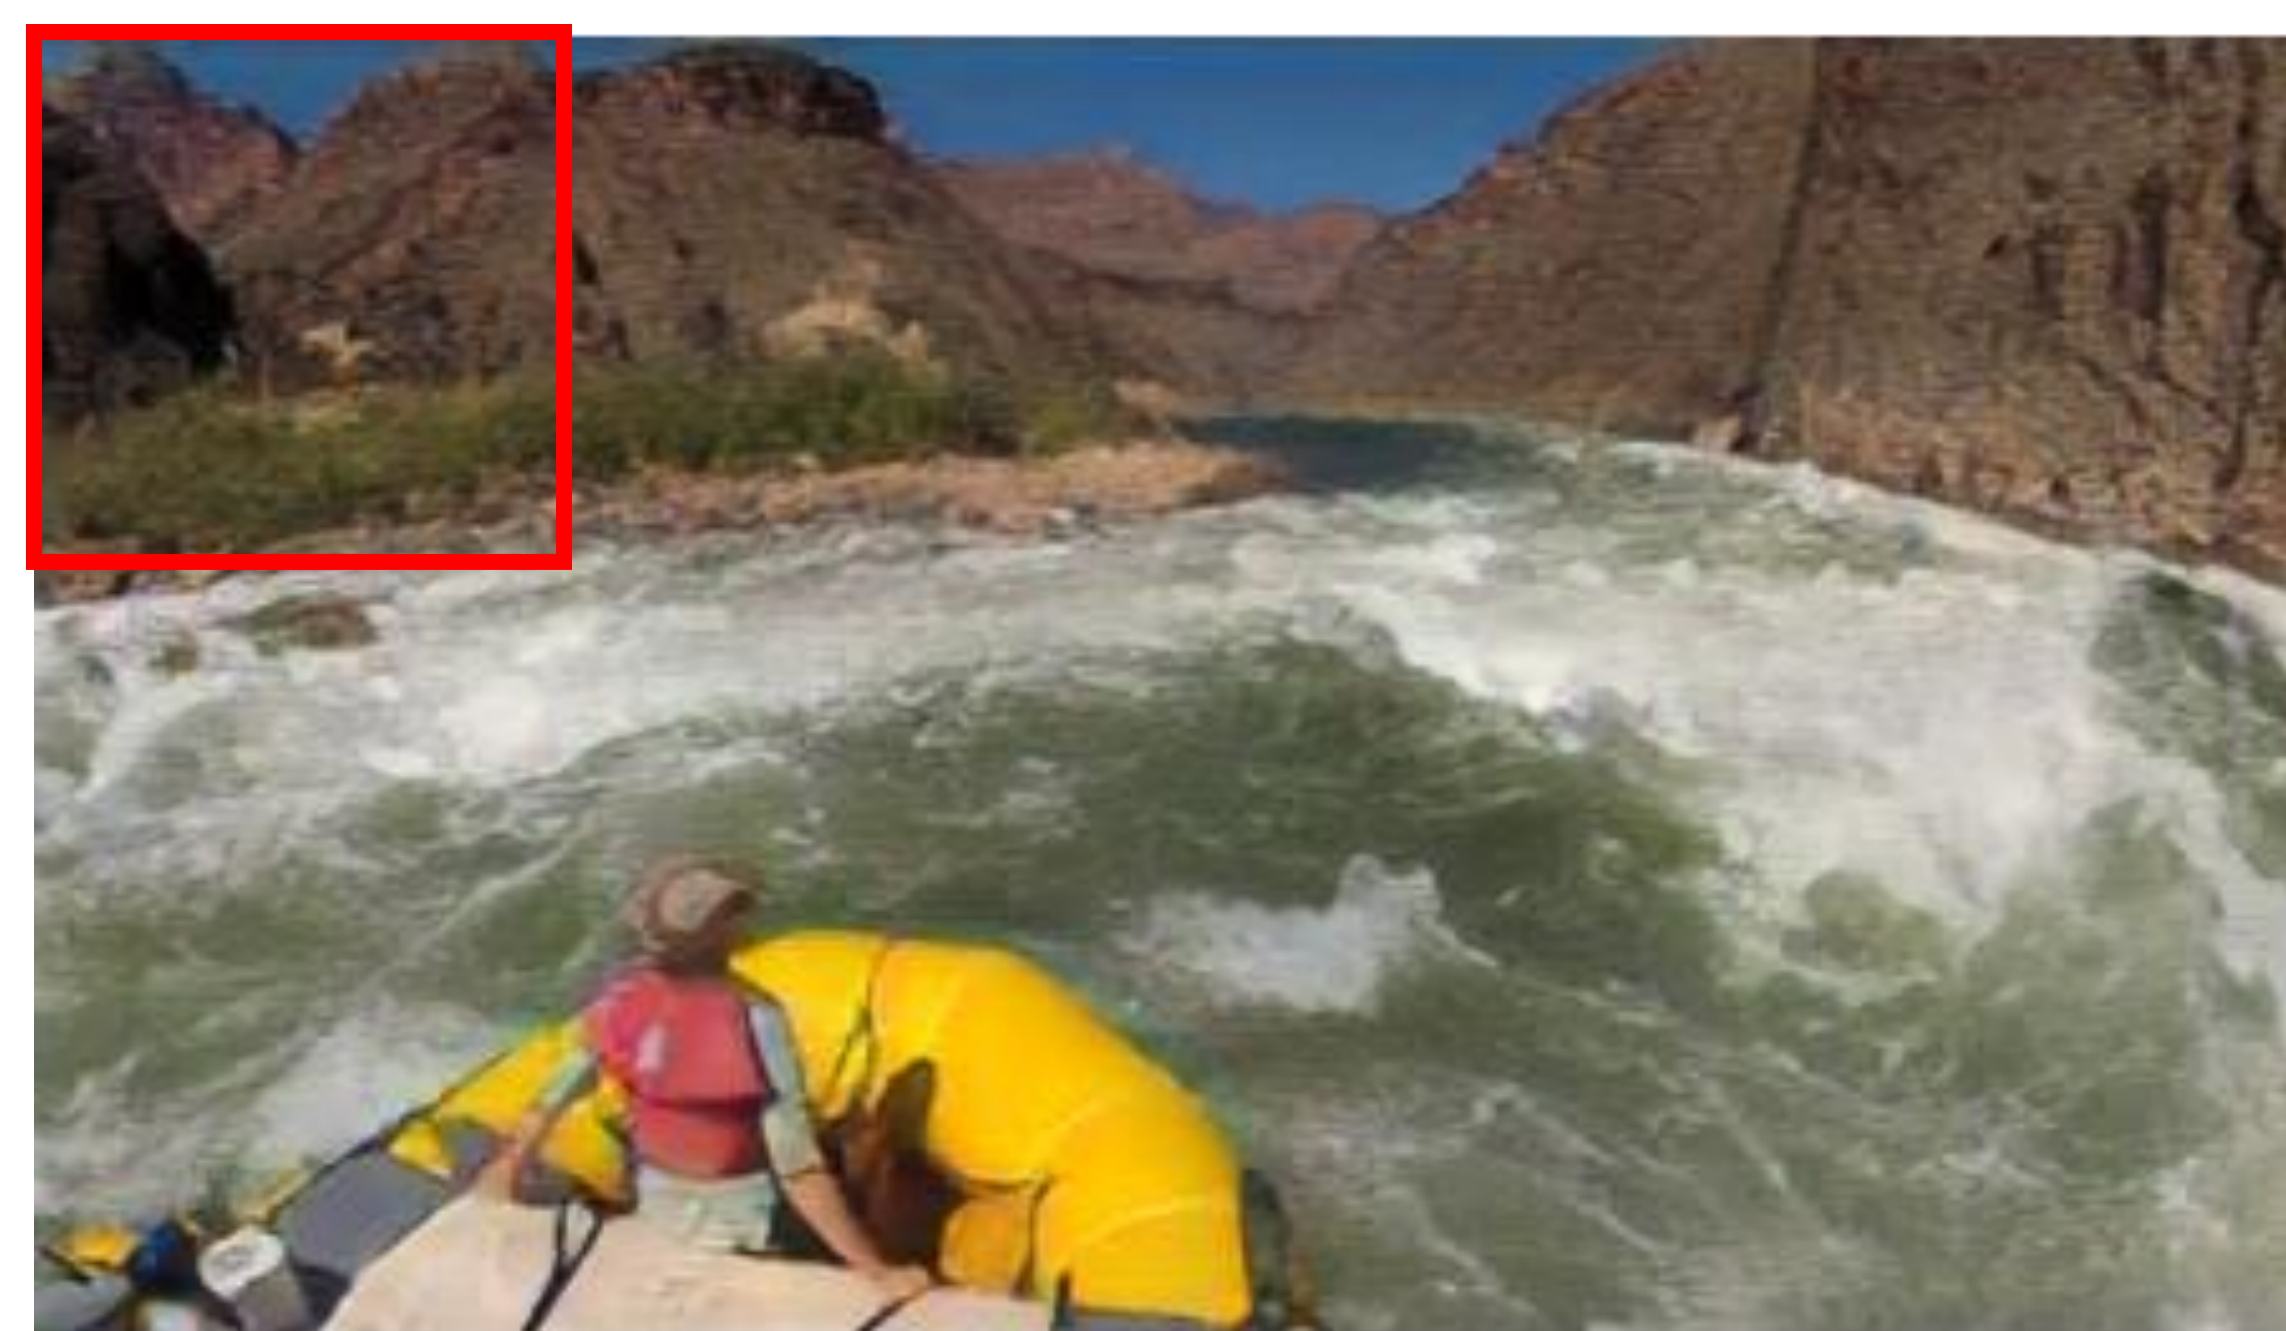

Video frame

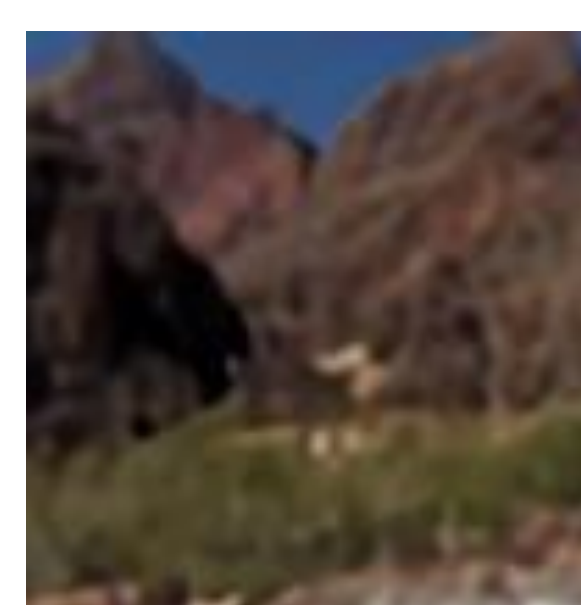

TMP

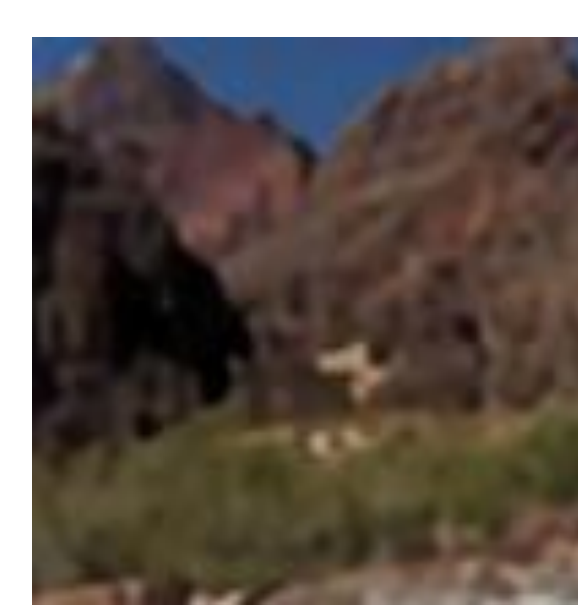

BasicVSR++

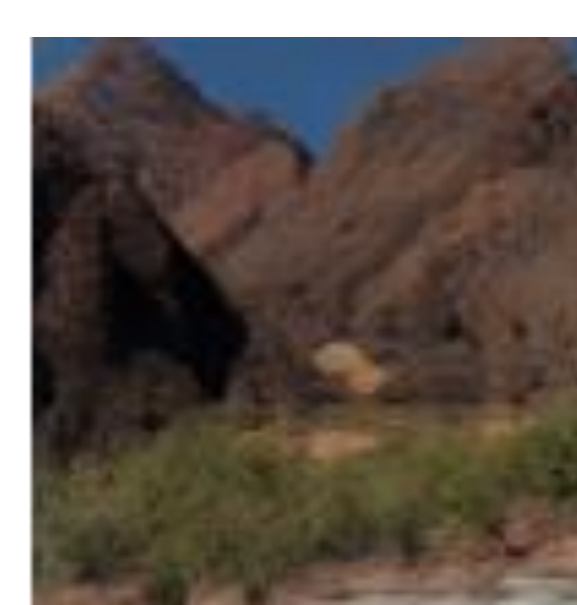

MGLD-VSR

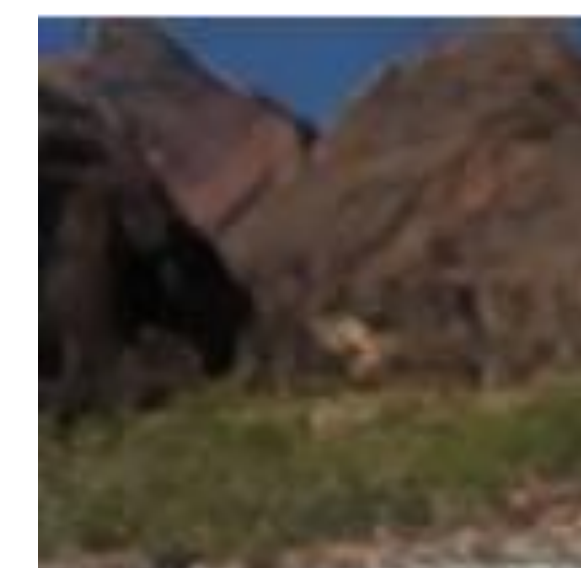

RealViFormer

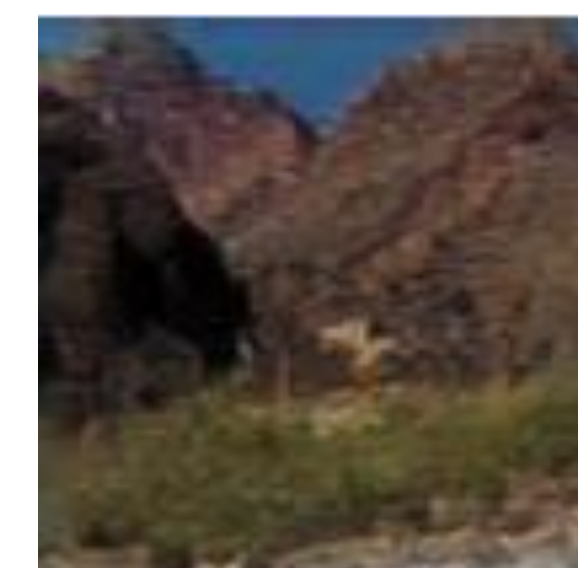

Ours

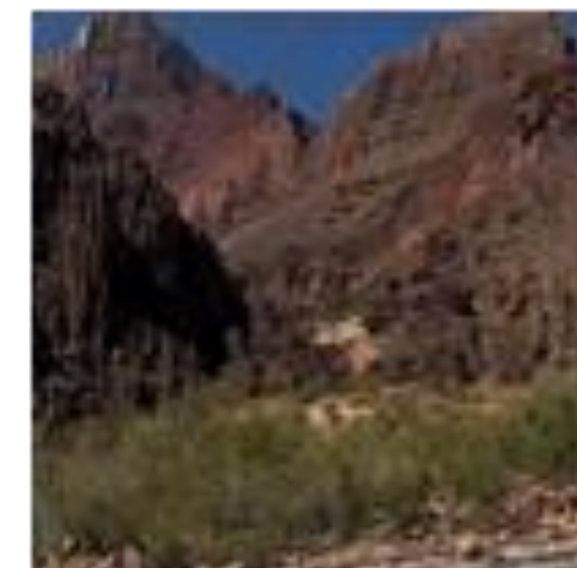

GT

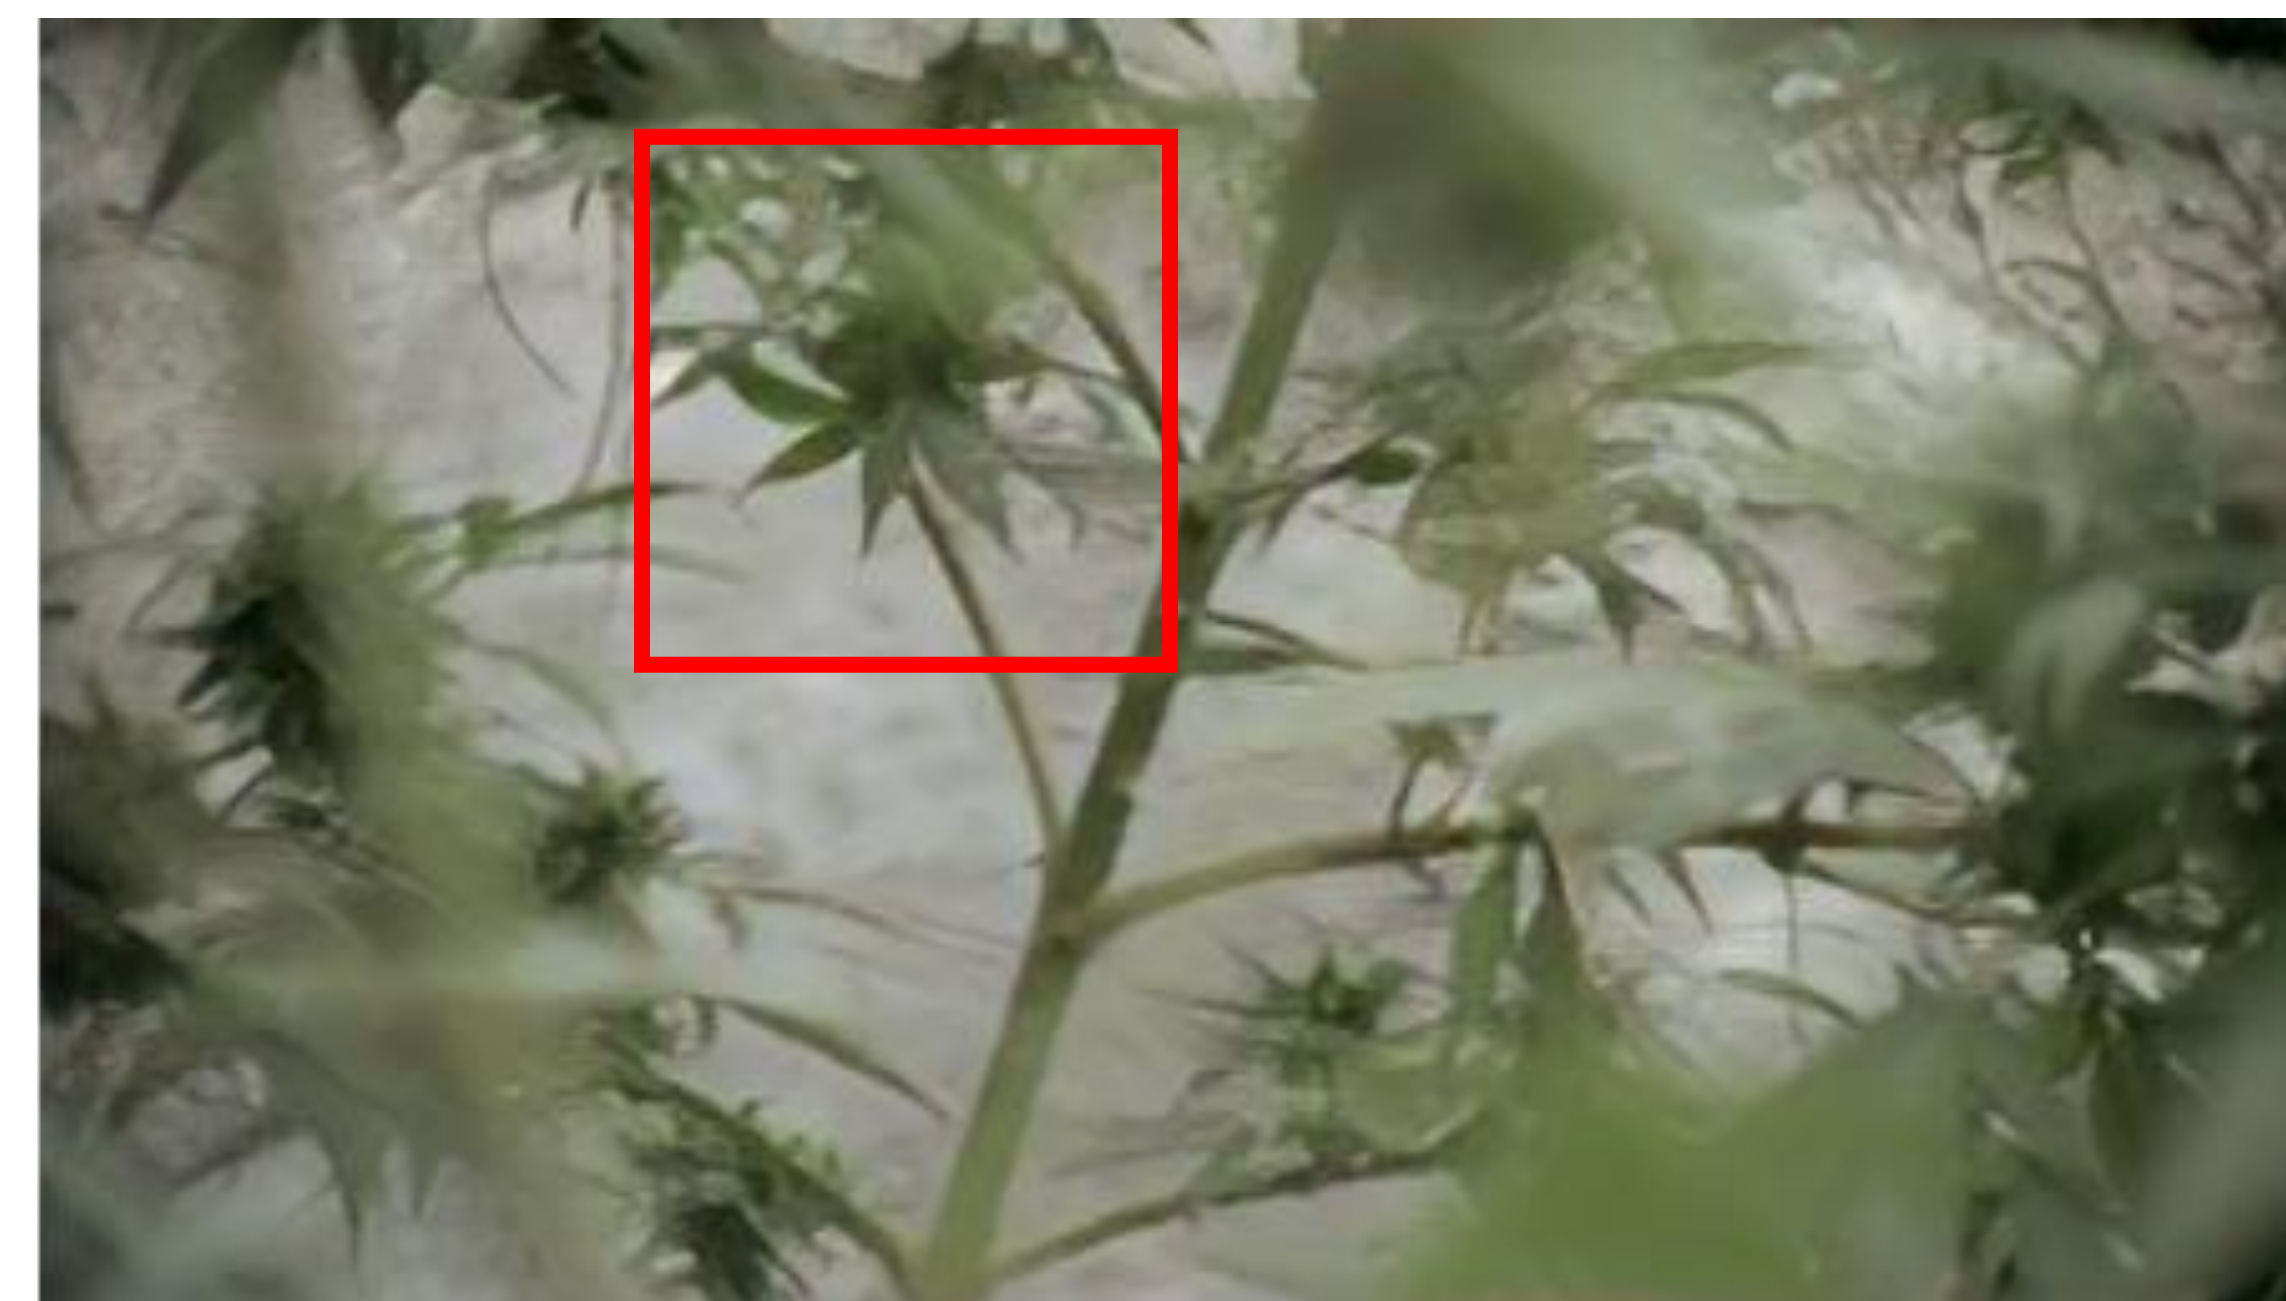

Video frame

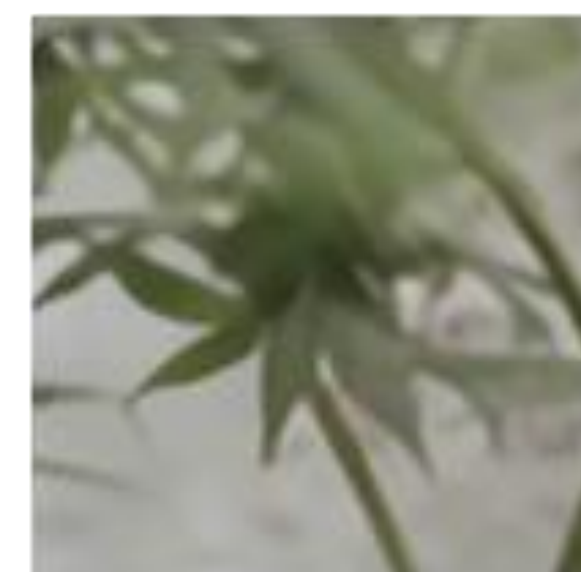

TMP

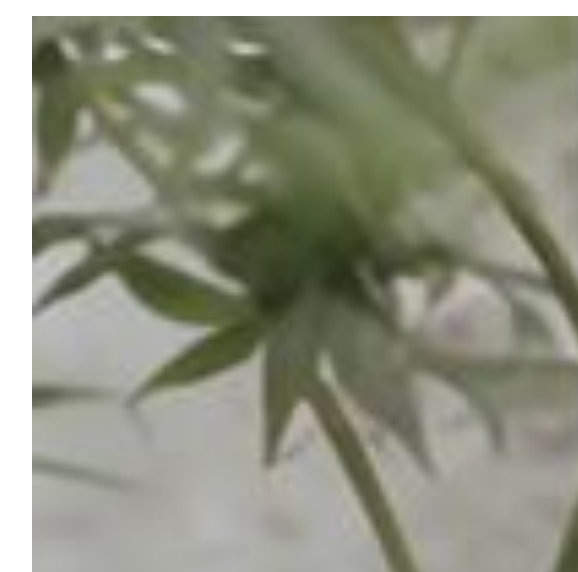

BasicVSR++

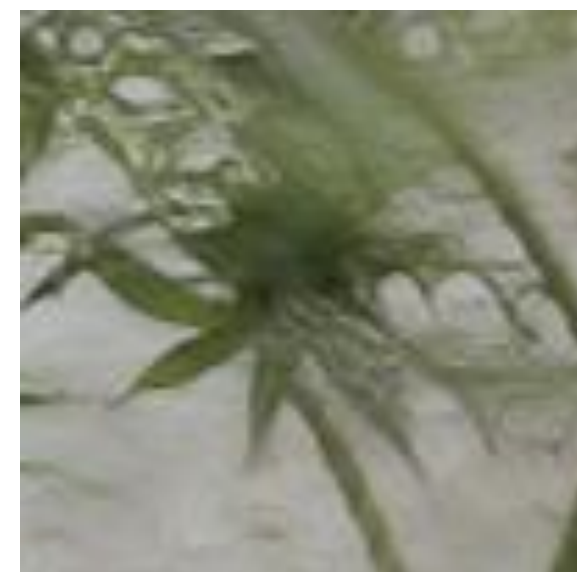

MGLD-VSR

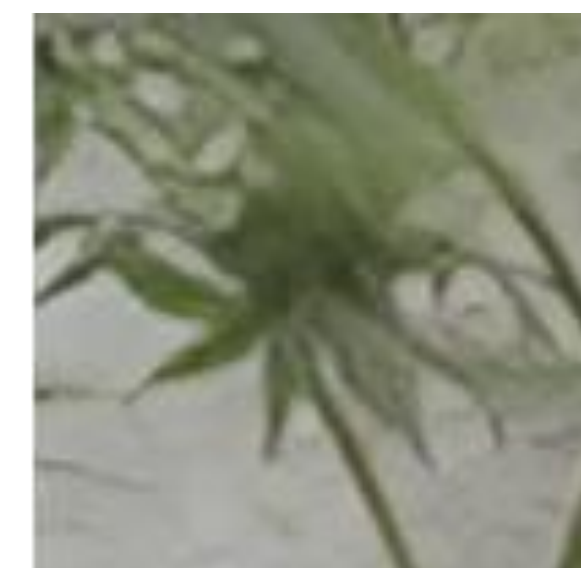

RealViFormer

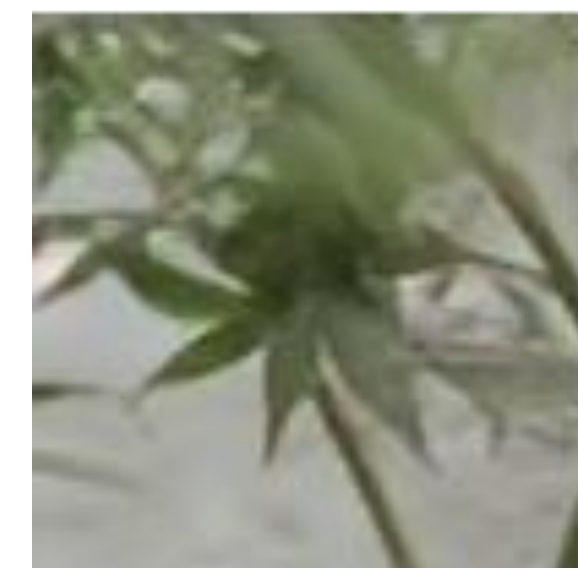

Ours

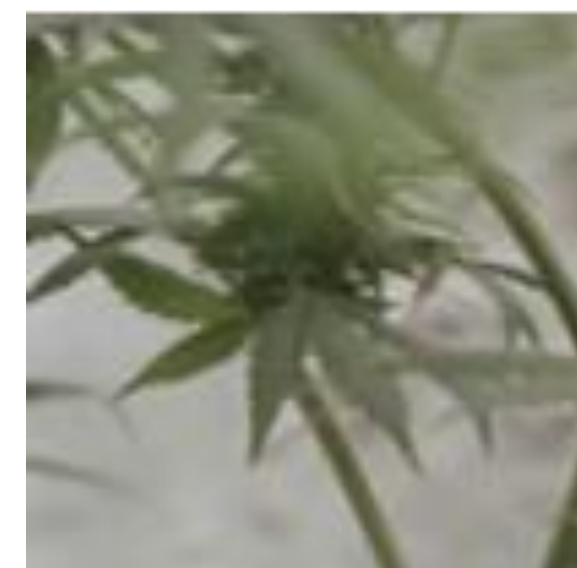

GT



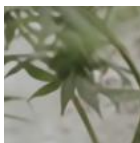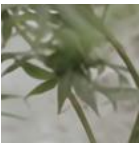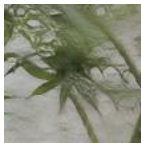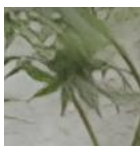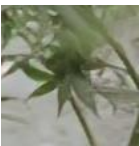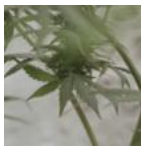

Supplement: Supplementary file 3 [file suppl_v3.pdf]
