# Supplementary material for: Stream-DiffVSR: Low-Latency Streamable Video Super-Resolution via Auto-Regressive Diffusion
Source: arXiv:2512.23709 source file (2026-08-31)

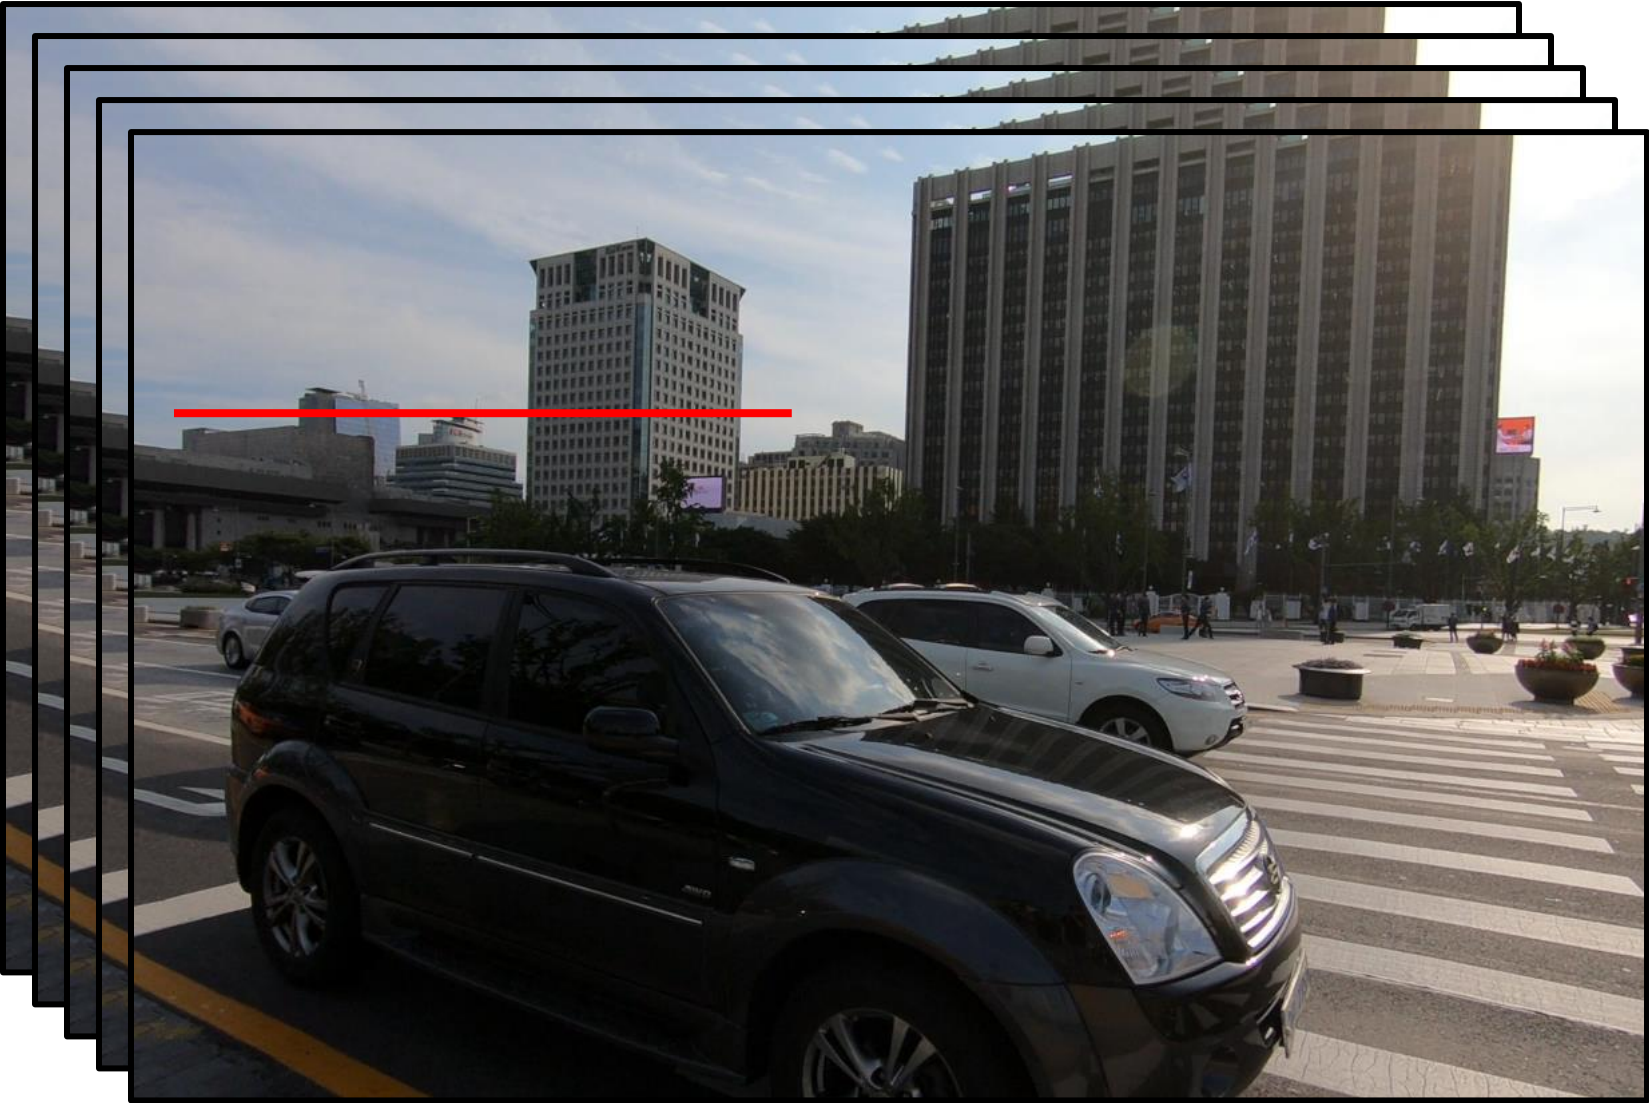

Time

Bicubic

MIA-VSR

MGLD-VSR

RealViFormer

X4-Upscaler

Ours

GT

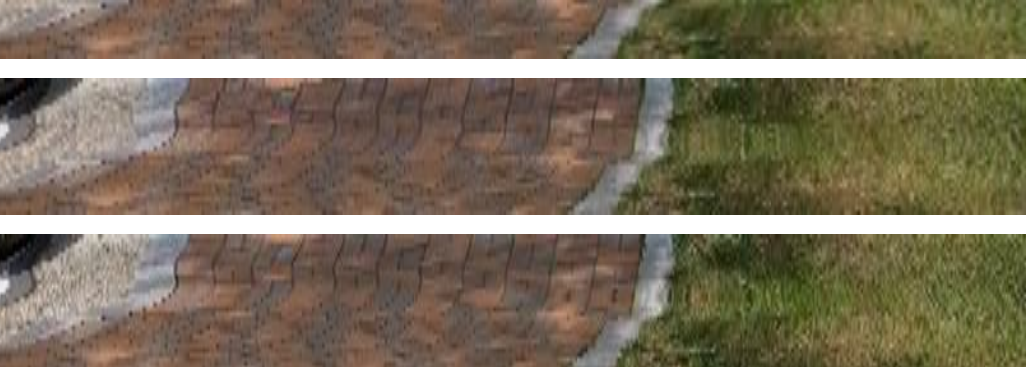

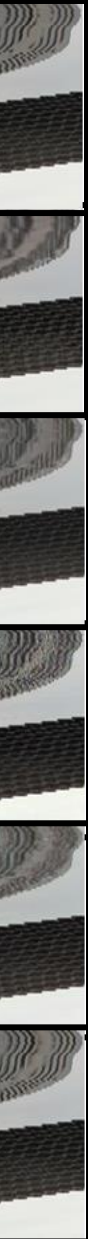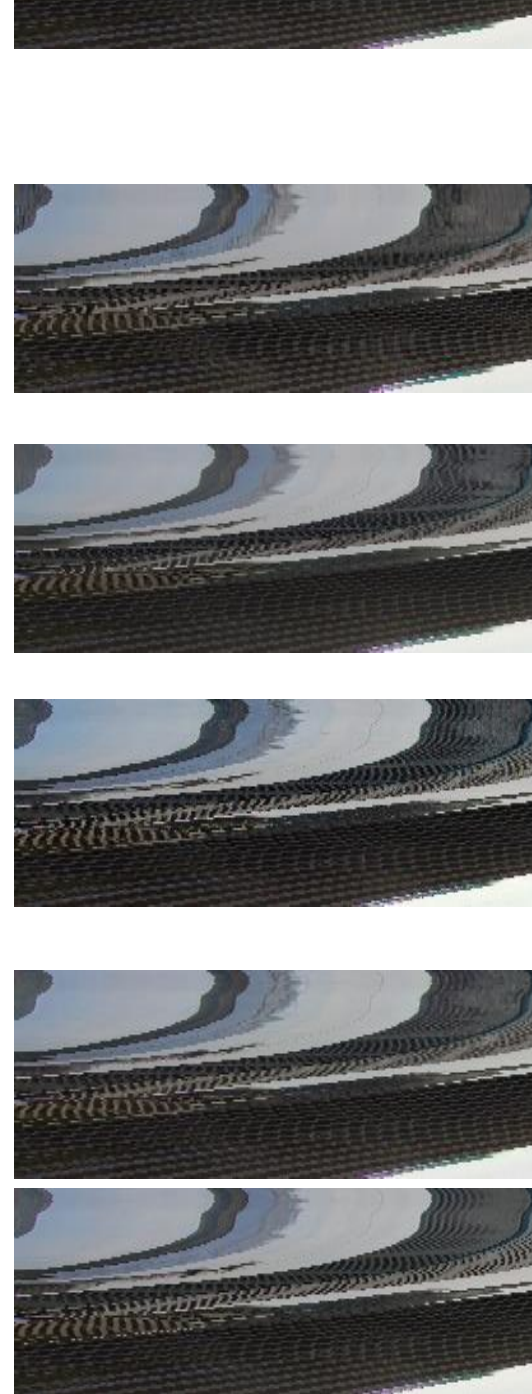

Supplement: Supplementary file 4 [file temporal.pdf]
