# Supplementary material for: Stream-DiffVSR: Low-Latency Streamable Video Super-Resolution via Auto-Regressive Diffusion
Source: arXiv:2512.23709 source file (2026-08-31)
Supplement: Supplementary file 6 [file table_reds4_suppl_bidirectional.tex]

\begin{table*}[t]
\caption{
\textbf{Quantitative comparison against bidirectional/offline methods on the REDS4 dataset with mean and standard deviation.} We compare CNN-, Transformer-, and diffusion-based approaches. Stream-DiffVSR shows superior perceptual quality, temporal consistency, and stability. All values are reported as \textit{mean ± std} over 4 videos. \(\uparrow\) / \(\downarrow\) denote higher/lower is better. \textbf{Dir.}: \textbf{B} = bidirectional/offline, \textbf{U} = unidirectional/online. Runtime is reported as the average per-frame inference time across all test sequences on an RTX 4090. \textbf{Latency-first} and \textbf{Latency-avg} measure first-frame and average latency; \textbf{tLP} and \textbf{tOF} are scaled by 100× and 10×. Best and second-best values are marked in \textcolor{red}{red} and \textcolor{blue}{blue}. For space reasons, the main paper reports the mean-only version; the full mean±std statistics are shown here.
}

\label{tab:vsr_online_comparison_reds4_suppl_bidirectional}
\vspace{-4mm}
\centering
\setlength{\tabcolsep}{5pt}
\renewcommand{\arraystretch}{1.1}
\resizebox{0.97\textwidth}{!}{%
\begin{tabular}{llcccccccccccccc}
\toprule
Dir. & Method & PSNR$\uparrow$ & SSIM$\uparrow$ & LPIPS$\downarrow$ & DISTS$\downarrow$ & MUSIQ$\uparrow$ & NIQE$\downarrow$ & NRQM$\uparrow$ & BRISQUE$\downarrow$ & tLP$\downarrow$ & tOF$\downarrow$ & Runtime (s)$\downarrow$ & latency-first (s)$\downarrow$ & latency-avg (s)$\downarrow$ \\
\midrule
\multicolumn{15}{c}{\textbf{CNN-based Methods}} \\
\midrule
-  & Bicubic & 25.501 ± 1.516 & 0.712 ± 0.062 & 0.460 ± 0.042 & 0.187 ± 0.013 & 27.362 ± 2.239 & 7.360 ± 0.120 & 3.459 ± 0.177 & 60.256 ± 1.828 & 21.603 ± 5.817 & 4.241 ± 5.765 & - & - & - \\
B  & BasicVSR++ & 32.386 ± 2.415 & 0.907 ± 0.029 & 0.132 ± 0.023 & 0.069 ± 0.012 & 67.002 ± 4.291 & 3.850 ± 0.439 & 6.363 ± 0.330 & 38.641 ± 5.224 & 9.017 ± 4.384 & 2.490 ± 4.440 & \textcolor{blue}{0.098} & 9.8 & 4.9 \\
B  & RealBasicVSR & 27.042 ± 1.865 & 0.778 ± 0.059 & 0.134 ± 0.016 & 0.060 ± 0.006 & 67.033 ± 4.283 & \textcolor{red}{2.530 ± 0.452} & 6.769 ± 0.242 & 18.046 ± 4.185 & 6.422 ± 4.726 & 4.759 ± 7.722 & \textcolor{red}{0.064} & \textcolor{blue}{6.4} & \textcolor{blue}{3.2} \\
\midrule
\multicolumn{15}{c}{\textbf{Transformer-based Methods}} \\
\midrule
B  & RVRT & \textcolor{blue}{32.701 ± 2.487} & \textcolor{blue}{0.911 ± 0.027} & 0.130 ± 0.022 & 0.067 ± 0.011 & \textcolor{blue}{67.251 ± 4.372} & 3.793 ± 0.463 & 6.366 ± 0.339 & 38.038 ± 5.779 & 9.133 ± 4.408 & \textcolor{blue}{2.421 ± 4.316} & 0.498 & 49.8 & 24.9 \\
B  & MIA-VSR & \textcolor{red}{32.790 ± 2.535} & \textcolor{red}{0.912 ± 0.028} & 0.123 ± 0.022 & 0.064 ± 0.011 & \textcolor{red}{68.140 ± 3.964} & 3.742 ± 0.472 & 6.451 ± 0.304 & 37.099 ± 5.668 & 8.870 ± 4.606 & \textcolor{red}{2.354 ± 4.026} & 0.768 & 0.768 & 0.768 \\
\midrule
\multicolumn{15}{c}{\textbf{Diffusion-based Methods}} \\
\midrule
B  & StableVSR & 27.928 ± 2.411 & 0.793 ± 0.063 & \textcolor{blue}{0.102 ± 0.015} & \textcolor{red}{0.047 ± 0.006} & 67.058 ± 3.797 & \textcolor{blue}{2.713 ± 0.456} & \textcolor{blue}{6.960 ± 0.211} & \textcolor{blue}{16.249 ± 4.133} & \textcolor{blue}{5.755 ± 4.618} & 2.742 ± 4.741 & 46.2 & 4620 & 2310 \\
B  & MGLD-VSR & 26.53 ± 1.939 & 0.749 ± 0.062 & 0.151 ± 0.019 & 0.065 ± 0.006 & 66.081 ± 4.027 & 2.972 ± 0.386 & 6.701 ± 0.202 & \textcolor{red}{15.291 ± 4.463} & 18.139 ± 8.772 & 5.910 ± 6.888 & 43.6 & 218 & 109 \\
U  & Ours & 27.256 ± 2.134 & 0.766 ± 0.062 & \textcolor{red}{0.099 ± 0.013} & \textcolor{blue}{0.062 ± 0.007} & 65.595 ± 3.982 & 3.114 ± 0.186 & \textcolor{red}{7.055 ± 0.257} & 17.117 ± 1.836 & \textcolor{red}{4.198 ± 3.795} & 3.638 ± 4.855 & 0.328 & \textcolor{red}{0.328} & \textcolor{red}{0.328} \\
\bottomrule
\end{tabular}%
}
\vspace{-2mm}
\end{table*}
