# Supplementary material for: Stream-DiffVSR: Low-Latency Streamable Video Super-Resolution via Auto-Regressive Diffusion
Source: arXiv:2512.23709 source file (2026-08-31)
Supplement: Supplementary file 7 [file table_reds4_suppl_unidirectional.tex]

\begin{table*}[t]
% \caption{
% \textbf{Quantitative comparison on the REDS4 dataset.} We evaluate the performance of various video super-resolution methods, including CNN-, Transformer-, and diffusion-based approaches on the REDS4 benchmark. Our AR-DiffVSR achieves superior perceptual quality and temporal consistency, while also demonstrating high output stability across different video sequences. All results are reported as \textit{mean ± standard deviation} across the 4 videos in the REDS4 dataset. Arrows in column headers indicate the direction of improvement: \(\uparrow\) means higher is better, \(\downarrow\) means lower is better. \textbf{Dir.} indicates the temporal direction used for each method: \textbf{B} for bidirectional/offline and \textbf{U} for unidirectional/online (past-only) models. Runtime denotes the average per-frame inference time (in seconds) on 720p videos using a single NVIDIA RTX 4090 GPU. Results are measured using the official implementations where available. Note: for readability, \textbf{tLP100 is scaled by 100×}, \textbf{tOF by 10×}, and \textbf{WarpErr by 1000×}. Best and second-best results are highlighted in \textcolor{red}{red} and \textcolor{blue}{blue}, respectively.}
\caption{
\textbf{Quantitative comparison against unidirectional/online methods on the REDS4 dataset with mean and standard deviation.}
}

\label{tab:vsr_online_comparison_reds4_suppl_unidirectional}
\vspace{-4mm}
\centering
\setlength{\tabcolsep}{5pt}
\renewcommand{\arraystretch}{1.1}
\resizebox{0.97\textwidth}{!}{%
\begin{tabular}{llcccccccccccccc}
\toprule
Dir. & Method & PSNR$\uparrow$ & SSIM$\uparrow$ & LPIPS$\downarrow$ & DISTS$\downarrow$ & MUSIQ$\uparrow$ & NIQE$\downarrow$ & NRQM$\uparrow$ & BRISQUE$\downarrow$ & tLP$\downarrow$ & tOF$\downarrow$ & Runtime (s)$\downarrow$ & latency-first (s)$\downarrow$ & latency-avg (s)$\downarrow$ \\
\midrule
\multicolumn{15}{c}{\textbf{CNN-based Methods}} \\
\midrule
-  & Bicubic & 25.501 ± 1.516 & 0.712 ± 0.062 & 0.460 ± 0.042 & 0.187 ± 0.013 & 27.362 ± 2.239 & 7.360 ± 0.120 & 3.459 ± 0.177 & 60.256 ± 1.828 & 21.603 ± 5.817 & 4.241 ± 5.765 & - & - & - \\
U  & TMP & \textcolor{red}{30.672 ± 2.317} & \textcolor{red}{0.871 ± 0.039} & 0.194 ± 0.039 & 0.090 ± 0.010 & 63.818 ± 4.129 & 4.378 ± 0.333 & 5.796 ± 0.312 & 43.394 ± 4.442 & 10.424 ± 5.654 & \textcolor{red}{2.480 ± 3.852} & \textcolor{red}{0.041} & \textcolor{red}{0.041} & \textcolor{red}{0.041} \\
\midrule
\multicolumn{15}{c}{\textbf{Transformer-based Methods}} \\
\midrule
U  & RealViformer & 26.763 ± 1.898 & 0.761 ± 0.062 & 0.129 ± 0.062 & 0.065 ± 0.004 & 64.585 ± 5.117 & \textcolor{blue}{2.731 ± 0.454} & 6.356 ± 0.079 & 17.272 ± 4.546 & 11.261 ± 5.613 & 11.782 ± 3.762 & \textcolor{blue}{0.099} & 9.9 & 4.95 \\
\midrule
\multicolumn{15}{c}{\textbf{Diffusion-based Methods}} \\
\midrule
U  & StableVSR* & 27.174 ± 2.449 & 0.763 ± 0.069 & \textcolor{blue}{0.111 ± 0.017} & \textcolor{red}{0.051 ± 0.006} & \textcolor{red}{66.428 ± 4.040} & \textcolor{red}{2.572 ± 0.356} & \textcolor{blue}{6.944 ± 0.211} & \textcolor{red}{15.805 ± 4.626} & \textcolor{blue}{11.107 ± 8.293} & 3.925 ± 4.561 & 46.2 & 4620 & 2310 \\
U  & Ours & \textcolor{blue}{27.256 ± 2.134} & \textcolor{blue}{0.766 ± 0.062} & \textcolor{red}{0.099 ± 0.013} & \textcolor{blue}{0.062 ± 0.007} & \textcolor{blue}{65.595 ± 3.982} & 3.114 ± 0.186 & \textcolor{red}{7.055 ± 0.257} & \textcolor{blue}{17.117 ± 1.836} & \textcolor{red}{4.198 ± 3.795} & \textcolor{blue}{3.638 ± 4.855} & 0.328 & \textcolor{blue}{0.328} & \textcolor{blue}{0.328} \\
\bottomrule
\end{tabular}%
}
\vspace{-2mm}
\end{table*}
