# Supplementary material for: Stream-DiffVSR: Low-Latency Streamable Video Super-Resolution via Auto-Regressive Diffusion
Source: arXiv:2512.23709 source file (2026-08-31)
Supplement: Supplementary file 8 [file table_videoLQ_suppl.tex]

\begin{table}[h]
\centering
\small 
\caption{\textbf{Quantitative comparison with memory-intensive baselines on the VideoLQ dataset under a single RTX Pro 6000.} Runtime is reported as the average per-frame inference time across all test sequences. \textbf{Latency-max} denotes the maximum end-to-end latency. \textbf{Peak-Mem} denotes the peak memory usage across all test sequences.
\textcolor{gray}{Gray-shaded entries are reported from FlashVSR.} \texttt{--} indicates unavailable results.} 
\label{tab:videolq_suppl_dit}
\vspace{-3mm}
\setlength{\tabcolsep}{2pt}
\resizebox{\columnwidth}{!}{%
\begin{tabular}{lcccccccc}
\toprule
Dir. & Method & NIQE$\downarrow$ & NRQM$\uparrow$ & BRISQUE$\downarrow$ & Runtime (s) & Latency-max (s) & Peak Mem (GB)\\
\midrule
B & VEhancer       & 6.221 ± 1.673 & 3.85 ± 1.107 & 48.1 ± 15.362 & 9.544 & 477.237 & 47.985 \\
B & SeedVR2          & \textcolor{blue}{4.661 ± 0.803} & \textcolor{blue}{5.523 ± 0.844} & 37.975 ± 8.257 & 1.126 & 56.28 & 76.094 \\
\rowcolor{black!10}
B & SeedVR2          & 5.205 & -- & -- & -- & -- & -- \\
B & UAV & 6.299 ± 0.723 & 3.652 ± 0.851 & 44.139 ± 8.898 & 8.081 & 404.07 & 55.897 \\
\rowcolor{black!10}
B & UAV & 4.889 & -- & -- & -- & -- & -- \\
B & DOVE           & 5.090 ± 0.961 & 5.214 ± 0.911 & \textcolor{blue}{36.631 ± 11.667} & 1.735 & 86.774 & 46.344 \\
U & FlashVSR & -- & -- & -- & -- & -- & OOM \\
\rowcolor{black!10}
U & FlashVSR & 3.803 & -- & -- & -- & -- & -- \\
U & FlashVSR-tiny & 4.569 ± 0.756 & 5.164 ± 0.888 & 42.514 ± 8.846 & \textcolor{red}{0.204} & 1.224 & \textcolor{blue}{44.180} \\
\rowcolor{black!10}
U & FlashVSR-tiny & 4.070 & -- & -- & -- & -- & -- \\
U & Ours            & \textcolor{red}{3.929 ± 0.64} & \textcolor{red}{6.140 ± 1.086} & \textcolor{red}{27.176 ± 5.664} & \textcolor{blue}{0.454} & \textcolor{red}{0.454} & \textcolor{red}{22.800} \\
\bottomrule
\end{tabular}%
}
\vspace{-4mm}
\end{table}
