# Supplementary material for: Stream-DiffVSR: Low-Latency Streamable Video Super-Resolution via Auto-Regressive Diffusion
Source: arXiv:2512.23709 source file (2026-08-31)
Supplement: Supplementary file 9 [file table_vimeo90K_suppl_bidirectional.tex]

\begin{table*}[t!]
\caption{
\textbf{Quantitative comparison on the Vimeo-90K-T dataset  with mean and standard deviation(bidirectional/offline).} Our Stream-DiffVSR achieves superior perceptual quality, temporal consistency, and substantially lower runtime. Results are reported as \textit{mean ± std} across the dataset, with runtime measured on 448×256 videos using an RTX 4090 GPU. Best and second-best results are shown in \textcolor{red}{red} and \textcolor{blue}{blue}. For space reasons, the main paper presents the mean-only version; the full mean±std statistics are provided here.}
\label{tab:vsr_online_comparison_vimeo_suppl_bidirectional}
\vspace{-4mm}
\centering
% \setlength{\tabcolsep}{5pt}
\renewcommand{\arraystretch}{1.1}
\resizebox{0.97\textwidth}{!}{%
\begin{tabular}{llccccccccccccc}
\toprule
Dir. & Method & PSNR$\uparrow$ & SSIM$\uparrow$ & LPIPS$\downarrow$ & DISTS$\downarrow$ & MUSIQ$\uparrow$ & NIQE$\downarrow$ & NRQM$\uparrow$ & BRISQUE$\downarrow$ & tLP$\downarrow$ & tOF$\downarrow$ & Runtime (s)$\downarrow$ & latency-first (s)$\downarrow$ & latency-avg (s)$\downarrow$ \\
\midrule
\multicolumn{15}{c}{\textbf{CNN-based Methods}} \\
\midrule
-  & Bicubic & $29.282 \pm 3.647$ & $0.864 \pm 0.061$ & $0.297 \pm 0.105$ & $0.209 \pm 0.044$ & $23.433 \pm 5.633$ & $8.735 \pm 0.397$ & $3.588 \pm 0.43$ & $61.714 \pm 4.599$ & $11.606 \pm 7.674$ & $2.49 \pm 1.645$ & - & - & - \\
B  & BasicVSR++ & $37.479 \pm 4.724$ & \textcolor{blue}{$0.956 \pm 0.033$} & $0.098 \pm 0.04$ & $0.117 \pm 0.024$ & $51.940 \pm 6.169$ & $7.077 \pm 1.111$ & $5.509 \pm 3.514$ & $47.792 \pm 12.514$ & \textcolor{red}{$4.691 \pm 5.013$} & $1.57 \pm 0.974$ & \textcolor{blue}{0.012} & 0.084 & 0.042 \\
B  & RealBasicVSR & $29.388 \pm 2.692$ & $0.857 \pm 0.059$ & $0.156 \pm 0.113$ & $0.149 \pm 0.06$ & \textcolor{blue}{$56.986 \pm 4.418$} & $5.069 \pm 0.464$ & \textcolor{blue}{$7.413 \pm 0.66$} & $23.822 \pm 10.19$ & $10.947 \pm 14.292$ & $3.46 \pm 2.446$ & \textcolor{red}{0.008} & \textcolor{blue}{0.056} & \textcolor{red}{0.028} \\
\midrule
\multicolumn{15}{c}{\textbf{Transformer-based Methods}} \\
\midrule
B  & RVRT & \textcolor{red}{$ 37.815 \pm 5.049 $} & $ 0.955 \pm 0.033 $ & $0.093 \pm 0.05$ & \textcolor{blue}{$0.105 \pm 0.023$} & $49.937 \pm 6.509$ & $7.205 \pm 1.005$ & $5.393 \pm 0.992$ & $48.352 \pm 12.147$ & $4.873 \pm 6.486$ & \textcolor{blue}{$1.429 \pm 1.079$} & 0.061 & 0.427 & 0.213 \\
B  & MIA-VSR & \textcolor{blue}{$ 37.598 \pm 4.724 $} & \textcolor{red}{$ 0.957 \pm 0.032 $} & \textcolor{blue}{$0.086 \pm 0.039$} & \textcolor{red}{$0.101 \pm 0.025$} & $51.402 \pm 6.522$ & $7.116 \pm 1.158$ & $5.569 \pm 1.249$ & $47.865 \pm 13.17$ & \textcolor{blue}{$4.696 \pm 5.874$} & \textcolor{red}{$1.419 \pm 0.997$} & 0.096 & 0.096 & 0.096 \\
\midrule
\multicolumn{15}{c}{\textbf{Diffusion-based Methods}} \\
\midrule
B  & StableVSR & $ 31.823 \pm 3.686 $ & $ 0.878 \pm 0.058 $ & $0.095 \pm 0.044$ & $0.111 \pm 0.025$ & $54.582 \pm 6.111$ & \textcolor{blue}{$4.745 \pm 0.857$} & $7.265 \pm 1.427$ & \textcolor{red}{$20.039 \pm 6.398$} & $26.224 \pm 9.042$ & $3.108 \pm 2.794$ & 5.749 & 40.243 & 20.121 \\
B  & MGLD-VSR & $ 29.651 \pm 2.354 $ & $ 0.865 \pm 0.057 $ & $0.151 \pm 0.076$ & $0.137 \pm 0.032$ & \textcolor{red}{$57.788 \pm 3.876$} & $5.340 \pm 0.798$ & $7.217 \pm 0.814$ & \textcolor{blue}{$20.761 \pm 8.394$} & $12.550 \pm 10.504$ & $4.661 \pm 3.449$ & 5.426 & 27.130 & 13.560 \\
U  & Ours & $ 32.593 \pm 3.82 $ & $ 0.900 \pm 0.060 $ & \textcolor{red}{$0.056 \pm 0.035$} & \textcolor{blue}{$0.105 \pm 0.017$} & $52.755 \pm 6.017$ & \textcolor{red}{$4.403 \pm 1.02$} & \textcolor{red}{$7.672 \pm 1.476$} & $29.297 \pm 10.007$ & \textcolor{red}{$4.307 \pm 4.359$} & $2.689 \pm 1.619$ & 0.041 & \textcolor{red}{0.041} & \textcolor{blue}{0.041} \\
\bottomrule
\end{tabular}%
}
\vspace{-2mm}
\end{table*}
