# Supplementary material for: Stream-DiffVSR: Low-Latency Streamable Video Super-Resolution via Auto-Regressive Diffusion
Source: arXiv:2512.23709 source file (2026-08-31)
Supplement: Supplementary file 10 [file table_vimeo90K_suppl_unidirectional.tex]

\begin{table*}[t!]
\caption{
\textbf{Quantitative comparison on the Vimeo-90K-T dataset with mean and standard deviation(unidirectional/online).}}
\label{tab:vsr_online_comparison_vimeo_suppl_unidirectional}
\vspace{-4mm}
\centering
% \setlength{\tabcolsep}{5pt}
\renewcommand{\arraystretch}{1.1}
\resizebox{0.97\textwidth}{!}{%
\begin{tabular}{llccccccccccccc}
\toprule
Dir. & Method & PSNR$\uparrow$ & SSIM$\uparrow$ & LPIPS$\downarrow$ & DISTS$\downarrow$ & MUSIQ$\uparrow$ & NIQE$\downarrow$ & NRQM$\uparrow$ & BRISQUE$\downarrow$ & tLP$\downarrow$ & tOF$\downarrow$ & Runtime (s)$\downarrow$ & latency-first (s)$\downarrow$ & latency-avg (s)$\downarrow$ \\
\midrule
\multicolumn{15}{c}{\textbf{CNN-based Methods}} \\
\midrule
-  & Bicubic & $29.282 \pm 3.647$ & $0.864 \pm 0.061$ & $0.297 \pm 0.105$ & $0.209 \pm 0.044$ & $23.433 \pm 5.633$ & $8.735 \pm 0.397$ & $3.588 \pm 0.43$ & $61.714 \pm 4.599$ & $11.606 \pm 7.674$ & $2.49 \pm 1.645$ & - & - & - \\
U  & TMP & \textcolor{red}{$ 36.482 \pm 4.672 $} & \textcolor{red}{$ 0.946 \pm 0.039 $} & $0.109 \pm 0.057$ & $0.118 \pm 0.027$ & $48.374 \pm 6.31$ & $7.368 \pm 0.909$ & $5.096 \pm 0.891$ & $49.192 \pm 11.55$ & \textcolor{red}{$4.870 \pm 5.177$} & \textcolor{red}{$1.603 \pm 1.011$} & \textcolor{red}{0.006} & \textcolor{red}{0.006} & \textcolor{red}{0.006} \\
\midrule
\multicolumn{15}{c}{\textbf{Transformer-based Methods}} \\
\midrule
U  & RealViformer & $ 30.291 \pm 2.518 $ & $ 0.877 \pm 0.055 $ & $0.130 \pm 0.061$ & $0.140 \pm 0.03$ & \textcolor{red}{$53.107 \pm 3.65$} & $5.515 \pm 0.486$ & $6.711 \pm 0.889$ & \textcolor{blue}{$24.628 \pm 7.933$} & $8.232 \pm 6.864$ & $2.769 \pm 1.909$ & \textcolor{blue}{0.013} & 0.091 & 0.045 \\
\midrule
\multicolumn{15}{c}{\textbf{Diffusion-based Methods}} \\
\midrule
U  & StableVSR* & $ 31.729 \pm 3.698 $ & $ 0.875 \pm 0.061 $ & \textcolor{red}{$0.098 \pm 0.049$} & \textcolor{blue}{$0.113 \pm 0.026$} & \textcolor{red}{$54.447 \pm 6.008$} & \textcolor{blue}{$4.698 \pm 0.853$} & \textcolor{blue}{$7.280 \pm 1.444$} & \textcolor{red}{$19.836 \pm 6.131$} & $30.858 \pm 13.166$ & $3.144 \pm 2.845$ & 5.749 & 40.243 & 20.121 \\
U  & Ours & \textcolor{red}{$ 32.593 \pm 3.82 $} & \textcolor{blue}{$ 0.900 \pm 0.060 $} & \textcolor{red}{$0.056 \pm 0.035$} & \textcolor{blue}{$0.105 \pm 0.017$} & $52.755 \pm 6.017$ & \textcolor{red}{$4.403 \pm 1.02$} & \textcolor{red}{$7.672 \pm 1.476$} & $29.297 \pm 10.007$ & \textcolor{red}{$4.307 \pm 4.359$} & \textcolor{blue}{$2.689 \pm 1.619$} & 0.041 & \textcolor{blue}{0.041} & \textcolor{blue}{0.041} \\
\bottomrule
\end{tabular}%
}
\vspace{-2mm}
\end{table*}
